# Supplementary material for: Statistical methods for Mendelian models with multiple genes and cancers
Source: arXiv:2108.12504 ancillary file (2022-05-07)
Supplement: Supplementary file 1 [file supplement.pdf]

# Additional figures, tables, and discussion for "Statistical methods for Mendelian models with multiple genes and cancers"

Jane W. Liang, Gregory E. Idos, Christine Hong, Stephen B. Gruber, Giovanni Parmigiani, and Danielle Braun

## S1 Back-Compatibility Simulations

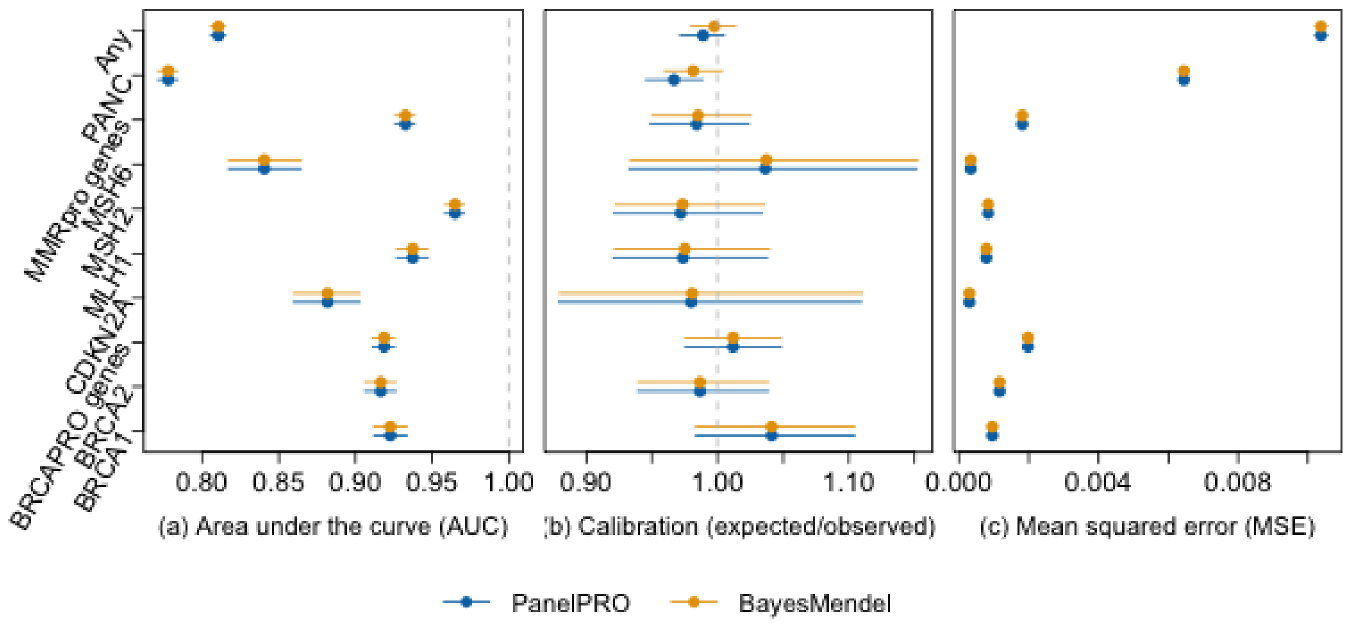


Figure S1: AUC, calibration, and MSE from fitting BRCAPRO, MMRpro, Pancpro, and Melapro using the PanelPRO (blue) and BayesMendel (orange) packages. "BRCAPRO genes" and "MMRpro genes" indicate any of the genes in BRCAPRO (BRCA1, BRCA2) and MMRpro (MLH1, MSH2, MSH6), respectively. "Any" indicates any of the seven genes that are included in BRCAPRO, MMRpro, Pancpro, and Melapro. 95% bootstrap percentile confidence intervals are also shown.

Table S1: AUC, calibration, and MSE from fitting BRCAPRO, MMRpro, Pancpro, and Melapro using the PanelPRO and BayesMendel packages. "BRCAPRO genes" and "MMRpro genes" indicate any of the genes in BRCAPRO (BRCA1, BRCA2) and MMRpro (MLH1, MSH2, MSH6), respectively. "Any" indicates any of the seven genes that are included in BRCAPRO, MMRpro, Pancpro, and Melapro. 95% bootstrap percentile confidence intervals are also reported.

(a) Area under the curve (AUC).

| Gene | Model | Estimate | Bootstrap 2.5% | Bootstrap 97.5% |
|---|---|---|---|---|
| BRCA1 | PanelPRO | 0.92272 | 0.91216 | 0.93352 |
| | BayesMendel | 0.92272 | 0.91216 | 0.93352 |
| BRCA2 | PanelPRO | 0.91649 | 0.90619 | 0.92610 |
| | BayesMendel | 0.91649 | 0.90619 | 0.92610 |
| BRCAPRO genes | PanelPRO | 0.91870 | 0.91119 | 0.92554 |
| | BayesMendel | 0.91870 | 0.91119 | 0.92554 |
| CDKN2A | PanelPRO | 0.88180 | 0.85950 | 0.90284 |
| | BayesMendel | 0.88180 | 0.85949 | 0.90284 |
| MLH1 | PanelPRO | 0.93736 | 0.92680 | 0.94734 |
| | BayesMendel | 0.93736 | 0.92680 | 0.94734 |
| MSH2 | PanelPRO | 0.96490 | 0.95803 | 0.97085 |
| | BayesMendel | 0.96489 | 0.95802 | 0.97084 |
| MSH6 | PanelPRO | 0.84057 | 0.81733 | 0.86441 |
| | BayesMendel | 0.84057 | 0.81732 | 0.86441 |
| MMRpro genes | PanelPRO | 0.93259 | 0.92566 | 0.93867 |
| | BayesMendel | 0.93258 | 0.92566 | 0.93866 |
| PANC | PanelPRO | 0.77801 | 0.77121 | 0.78419 |
| | BayesMendel | 0.77800 | 0.77114 | 0.78417 |
| Any | PanelPRO | 0.81066 | 0.80557 | 0.81498 |
| | BayesMendel | 0.81062 | 0.80552 | 0.81492 |

Table S1: (continued from previous page)

(b) Calibration (expected divided by observed number of events).

| Gene | Model | Estimate | Bootstrap 2.5% | Bootstrap 97.5% |
|---|---|---|---|---|
| BRCA1 | PanelPRO | 1.04119 | 0.98344 | 1.10426 |
| | BayesMendel | 1.04119 | 0.98344 | 1.10426 |
| BRCA2 | PanelPRO | 0.98663 | 0.93918 | 1.03868 |
| | BayesMendel | 0.98663 | 0.93918 | 1.03868 |
| BRCAPRO genes | PanelPRO | 1.01183 | 0.97516 | 1.04833 |
| | BayesMendel | 1.01183 | 0.97516 | 1.04833 |
| CDKN2A | PanelPRO | 0.97987 | 0.87915 | 1.10940 |
| | BayesMendel | 0.98059 | 0.87980 | 1.11020 |
| MLH1 | PanelPRO | 0.97369 | 0.92030 | 1.03801 |
| | BayesMendel | 0.97513 | 0.92165 | 1.03954 |
| MSH2 | PanelPRO | 0.97185 | 0.92082 | 1.03399 |
| | BayesMendel | 0.97338 | 0.92225 | 1.03566 |
| MSH6 | PanelPRO | 1.03634 | 0.93277 | 1.15154 |
| | BayesMendel | 1.03719 | 0.93354 | 1.15250 |
| MMRpro genes | PanelPRO | 0.98403 | 0.94876 | 1.02409 |
| | BayesMendel | 0.98525 | 0.94996 | 1.02540 |
| PANC | PanelPRO | 0.96688 | 0.94534 | 0.98888 |
| | BayesMendel | 0.98137 | 0.95955 | 1.00373 |
| Any | PanelPRO | 0.98889 | 0.97156 | 1.00499 |
| | BayesMendel | 0.99751 | 0.98000 | 1.01376 |

(c) Mean squared error (MSE).

| Gene | Model | Estimate | Bootstrap 2.5% | Bootstrap 97.5% |
|---|---|---|---|---|
| BRCA1 | PanelPRO | 0.00096 | 0.00090 | 0.00101 |
| | BayesMendel | 0.00096 | 0.00090 | 0.00101 |
| BRCA2 | PanelPRO | 0.00116 | 0.00111 | 0.00122 |
| | BayesMendel | 0.00116 | 0.00111 | 0.00122 |
| BRCAPRO genes | PanelPRO | 0.00198 | 0.00191 | 0.00205 |
| | BayesMendel | 0.00198 | 0.00191 | 0.00205 |
| CDKN2A | PanelPRO | 0.00030 | 0.00026 | 0.00033 |
| | BayesMendel | 0.00030 | 0.00026 | 0.00033 |
| MLH1 | PanelPRO | 0.00078 | 0.00073 | 0.00083 |
| | BayesMendel | 0.00078 | 0.00073 | 0.00083 |
| MSH2 | PanelPRO | 0.00084 | 0.00078 | 0.00089 |
| | BayesMendel | 0.00084 | 0.00078 | 0.00089 |
| MSH6 | PanelPRO | 0.00034 | 0.00030 | 0.00037 |
| | BayesMendel | 0.00034 | 0.00030 | 0.00037 |
| MMRpro genes | PanelPRO | 0.00181 | 0.00174 | 0.00189 |
| | BayesMendel | 0.00181 | 0.00174 | 0.00189 |
| PANC | PanelPRO | 0.00645 | 0.00631 | 0.00659 |
| | BayesMendel | 0.00645 | 0.00631 | 0.00659 |
| Any | PanelPRO | 0.01037 | 0.01020 | 0.01055 |
| | BayesMendel | 0.01037 | 0.01020 | 0.01055 |

## S2 PanelPRO-5BC Simulations

Table S2: AUC, calibration, and MSE for the full PanelPRO-5BC model and its BRCAPRO submodel evaluated on 1,000,000 families simulated based on PanelPRO-5BC, with and without risk modifiers. "BRCAPRO genes" indicates any of the genes in BRCAPRO (BRCA1, BRCA2), and "Any" indicates any of the five genes in PanelPRO-5BC. 95% bootstrap percentile confidence intervals are also reported.

(a) Area under the curve (AUC).

| Gene | Model | Risk Modifiers | Estimate | Bootstrap 2.5% | Bootstrap 97.5% |
|---|---|---|---|---|---|
| ATM | Full model | No | 0.59970 | 0.59049 | 0.60898 |
| | Full model | Yes | 0.59981 | 0.59057 | 0.60906 |
| BRCA1 | Full model | No | 0.92351 | 0.91315 | 0.93273 |
| | Full model | Yes | 0.93144 | 0.92062 | 0.94133 |
| | Submodel | No | 0.92351 | 0.91315 | 0.93272 |
| | Submodel | Yes | 0.93142 | 0.92060 | 0.94131 |
| BRCA2 | Full model | No | 0.92575 | 0.91612 | 0.93403 |
| | Full model | Yes | 0.92641 | 0.91673 | 0.93492 |
| | Submodel | No | 0.92575 | 0.91612 | 0.93402 |
| | Submodel | Yes | 0.92641 | 0.91673 | 0.93493 |
| BRCAPRO genes | Full model | No | 0.92429 | 0.91770 | 0.93064 |
| | Full model | Yes | 0.92767 | 0.92068 | 0.93404 |
| | Submodel | No | 0.92428 | 0.91768 | 0.93063 |
| | Submodel | Yes | 0.92765 | 0.92066 | 0.93402 |
| CHEK2 | Full model | No | 0.55520 | 0.54767 | 0.56357 |
| | Full model | Yes | 0.55494 | 0.54740 | 0.56339 |
| PALB2 | Full model | No | 0.69119 | 0.67551 | 0.70701 |
| | Full model | Yes | 0.69079 | 0.67514 | 0.70667 |
| Any | Full model | No | 0.64650 | 0.64110 | 0.65165 |
| | Full model | Yes | 0.64695 | 0.64150 | 0.65209 |

Table S2: (continued from previous page)

(b) Calibration (expected divided by observed number of events).

| Gene | Model | Risk Modifiers | Estimate | Bootstrap 2.5% | Bootstrap 97.5% |
|---|---|---|---|---|---|
| ATM | Full model | No | 0.96840 | 0.93992 | 1.00131 |
| | Full model | Yes | 0.96863 | 0.94013 | 1.00157 |
| BRCA1 | Full model | No | 1.02008 | 0.96740 | 1.07724 |
| | Full model | Yes | 0.85052 | 0.80962 | 0.89787 |
| | Submodel | No | 1.01774 | 0.96508 | 1.07478 |
| | Submodel | Yes | 0.84938 | 0.80855 | 0.89674 |
| BRCA2 | Full model | No | 0.96981 | 0.92536 | 1.01929 |
| | Full model | Yes | 1.01486 | 0.96717 | 1.06478 |
| | Submodel | No | 0.96795 | 0.92361 | 1.01740 |
| | Submodel | Yes | 1.01296 | 0.96536 | 1.06279 |
| BRCAPRO genes | Full model | No | 1.00147 | 0.96720 | 1.03965 |
| | Full model | Yes | 0.95249 | 0.91949 | 0.98775 |
| | Submodel | No | 0.99169 | 0.95770 | 1.02948 |
| | Submodel | Yes | 0.94363 | 0.91085 | 0.97862 |
| CHEK2 | Full model | No | 0.99169 | 0.96512 | 1.01891 |
| | Full model | Yes | 0.99186 | 0.96526 | 1.01906 |
| PALB2 | Full model | No | 0.96141 | 0.90353 | 1.02390 |
| | Full model | Yes | 0.96185 | 0.90407 | 1.02433 |
| Any | Full model | No | 0.99102 | 0.97396 | 1.00871 |
| | Full model | Yes | 0.98173 | 0.96500 | 0.99924 |

(c) Mean squared error (MSE).

| Gene | Model | Risk Modifiers | Estimate | Bootstrap 2.5% | Bootstrap 97.5% |
|---|---|---|---|---|---|
| ATM | Full model | No | 0.00386 | 0.00374 | 0.00398 |
| | Full model | Yes | 0.00386 | 0.00374 | 0.00398 |
| BRCA1 | Full model | No | 0.00099 | 0.00093 | 0.00104 |
| | Full model | Yes | 0.00090 | 0.00085 | 0.00095 |
| | Submodel | No | 0.00099 | 0.00093 | 0.00104 |
| | Submodel | Yes | 0.00090 | 0.00085 | 0.00095 |
| BRCA2 | Full model | No | 0.00118 | 0.00112 | 0.00124 |
| | Full model | Yes | 0.00115 | 0.00109 | 0.00121 |
| | Submodel | No | 0.00118 | 0.00112 | 0.00124 |
| | Submodel | Yes | 0.00115 | 0.00109 | 0.00121 |
| BRCAPRO genes | Full model | No | 0.00202 | 0.00195 | 0.00210 |
| | Full model | Yes | 0.00198 | 0.00191 | 0.00206 |
| | Submodel | No | 0.00202 | 0.00195 | 0.00210 |
| | Submodel | Yes | 0.00198 | 0.00191 | 0.00206 |
| CHEK2 | Full model | No | 0.00513 | 0.00500 | 0.00527 |
| | Full model | Yes | 0.00513 | 0.00500 | 0.00527 |
| PALB2 | Full model | No | 0.00118 | 0.00111 | 0.00125 |
| | Full model | Yes | 0.00118 | 0.00111 | 0.00125 |
| Any | Full model | No | 0.01191 | 0.01170 | 0.01212 |
| | Full model | Yes | 0.01187 | 0.01166 | 0.01208 |

## S3 PanelPRO-11 Simulations

Table S3: AUC, calibration, and MSE for the full PanelPRO-11 model and its BayesMendel submodels BRCAPRO, MMRpro, and Melapro evaluated on 1,000,000 families simulated based on PanelPRO-11, with and without risk modifiers. "BRCAPRO genes", "MMRpro genes", and "Any BM" indicate any of the genes in BRCAPRO (BRCA1, BRCA2), MMRpro (MLH1, MSH2, MSH6), and any model in the BayesMendel package (BRCA1, BRCA2, MLH1, MSH2, MSH6, CDKN2A), respectively. "Any" indicates any of the eleven genes in PanelPRO-11. 95% bootstrap percentile confidence intervals are also reported.

(a) Area under the curve (AUC).

| Gene | Model | Risk Modifiers | Estimate | Bootstrap 2.5% | Bootstrap 97.5% |
|---|---|---|---|---|---|
| ATM | Full model | No | 0.63715 | 0.62847 | 0.64688 |
| | Full model | Yes | 0.63715 | 0.62850 | 0.64690 |
| BRCA1 | Full model | No | 0.92825 | 0.91939 | 0.93722 |
| | Full model | Yes | 0.94159 | 0.93337 | 0.94952 |
| | Submodel | No | 0.92553 | 0.91610 | 0.93471 |
| | Submodel | Yes | 0.93957 | 0.93085 | 0.94792 |
| BRCA2 | Full model | No | 0.93066 | 0.92211 | 0.93809 |
| | Full model | Yes | 0.93104 | 0.92249 | 0.93858 |
| | Submodel | No | 0.92642 | 0.91740 | 0.93445 |
| | Submodel | Yes | 0.92665 | 0.91757 | 0.93479 |
| BRCAPRO genes | Full model | No | 0.92943 | 0.92318 | 0.93547 |
| | Full model | Yes | 0.93316 | 0.92688 | 0.93892 |
| | Submodel | No | 0.92589 | 0.91938 | 0.93190 |
| | Submodel | Yes | 0.92965 | 0.92316 | 0.93551 |
| CDKN2A | Full model | No | 0.91396 | 0.89417 | 0.93228 |
| | Full model | Yes | 0.91363 | 0.89364 | 0.93196 |
| | Submodel | No | 0.84506 | 0.81849 | 0.87191 |
| | Submodel | Yes | 0.84506 | 0.81849 | 0.87191 |
| CHEK2 | Full model | No | 0.63884 | 0.63051 | 0.64687 |
| | Full model | Yes | 0.63870 | 0.63026 | 0.64681 |
| EPCAM | Full model | No | 0.99848 | 0.99712 | 0.99958 |
| | Full model | Yes | 0.99891 | 0.99797 | 0.99968 |
| MLH1 | Full model | No | 0.97091 | 0.96442 | 0.97703 |
| | Full model | Yes | 0.98141 | 0.97609 | 0.98658 |
| | Submodel | No | 0.95445 | 0.94474 | 0.96241 |
| | Submodel | Yes | 0.96969 | 0.96130 | 0.97673 |
| MSH2 | Full model | No | 0.97901 | 0.97384 | 0.98374 |
| | Full model | Yes | 0.98599 | 0.98120 | 0.99012 |
| | Submodel | No | 0.96273 | 0.95624 | 0.96890 |
| | Submodel | Yes | 0.97656 | 0.97068 | 0.98193 |
| MSH6 | Full model | No | 0.85549 | 0.83085 | 0.87974 |
| | Full model | Yes | 0.88721 | 0.86241 | 0.91091 |
| | Submodel | No | 0.81138 | 0.78446 | 0.83782 |
| | Submodel | Yes | 0.85436 | 0.82745 | 0.88081 |
| MMRpro genes | Full model | No | 0.95419 | 0.94836 | 0.95928 |
| | Full model | Yes | 0.96669 | 0.96166 | 0.97145 |
| | Submodel | No | 0.93532 | 0.92860 | 0.94138 |
| | Submodel | Yes | 0.95381 | 0.94738 | 0.95953 |
| PALB2 | Full model | No | 0.69181 | 0.67586 | 0.70905 |
| | Full model | Yes | 0.69156 | 0.67540 | 0.70854 |
| PMS2 | Full model | No | 0.56632 | 0.55240 | 0.58072 |
| | Full model | Yes | 0.63357 | 0.61895 | 0.64745 |
| Any BM | Full model | No | 0.91916 | 0.91422 | 0.92370 |
| | Full model | Yes | 0.93073 | 0.92610 | 0.93493 |
| | Submodel | No | 0.90364 | 0.89850 | 0.90846 |
| | Submodel | Yes | 0.91879 | 0.91367 | 0.92338 |
| Any | Full model | No | 0.69430 | 0.69034 | 0.69909 |
| | Full model | Yes | 0.70059 | 0.69647 | 0.70521 |

Table S3: (continued from previous page)

(b) Calibration (expected divided by observed number of events).

| Gene | Model | Risk Modifiers | Estimate | Bootstrap 2.5% | Bootstrap 97.5% |
|---|---|---|---|---|---|
| ATM | Full model | No | 0.98627 | 0.95630 | 1.01938 |
| | Full model | Yes | 0.98658 | 0.95650 | 1.01981 |
| BRCA1 | Full model | No | 1.01273 | 0.96276 | 1.06748 |
| | Full model | Yes | 0.85379 | 0.81262 | 0.89824 |
| | Submodel | No | 1.00959 | 0.95923 | 1.06452 |
| | Submodel | Yes | 0.85115 | 0.81033 | 0.89484 |
| BRCA2 | Full model | No | 1.00296 | 0.95526 | 1.05576 |
| | Full model | Yes | 1.04727 | 0.99773 | 1.10175 |
| | Submodel | No | 0.99809 | 0.95030 | 1.04934 |
| | Submodel | Yes | 1.04310 | 0.99354 | 1.09750 |
| BRCAPRO genes | Full model | No | 1.01781 | 0.98310 | 1.05425 |
| | Full model | Yes | 0.97029 | 0.93772 | 1.00393 |
| | Submodel | No | 1.00257 | 0.96865 | 1.03859 |
| | Submodel | Yes | 0.95653 | 0.92457 | 0.98912 |
| CDKN2A | Full model | No | 0.99774 | 0.89985 | 1.12565 |
| | Full model | Yes | 0.99811 | 0.90018 | 1.12592 |
| | Submodel | No | 0.99158 | 0.89402 | 1.11647 |
| | Submodel | Yes | 0.99158 | 0.89402 | 1.11647 |
| CHEK2 | Full model | No | 0.95887 | 0.93569 | 0.98478 |
| | Full model | Yes | 0.95903 | 0.93584 | 0.98493 |
| EPCAM | Full model | No | 0.82103 | 0.60819 | 1.15672 |
| | Full model | Yes | 0.91597 | 0.68873 | 1.25859 |
| MLH1 | Full model | No | 1.00885 | 0.95408 | 1.06722 |
| | Full model | Yes | 0.99085 | 0.93929 | 1.04719 |
| | Submodel | No | 1.00876 | 0.95085 | 1.06938 |
| | Submodel | Yes | 0.99690 | 0.94107 | 1.05572 |
| MSH2 | Full model | No | 0.97349 | 0.92525 | 1.02685 |
| | Full model | Yes | 0.96868 | 0.92174 | 1.02110 |
| | Submodel | No | 0.97625 | 0.92211 | 1.03135 |
| | Submodel | Yes | 0.96643 | 0.91909 | 1.02008 |
| MSH6 | Full model | No | 1.07297 | 0.96656 | 1.18515 |
| | Full model | Yes | 1.07705 | 0.97189 | 1.19479 |
| | Submodel | No | 1.08344 | 0.97690 | 1.19712 |
| | Submodel | Yes | 1.09476 | 0.98803 | 1.20888 |
| MMRpro genes | Full model | No | 1.00979 | 0.97323 | 1.04471 |
| | Full model | Yes | 1.00155 | 0.96553 | 1.03519 |
| | Submodel | No | 1.00567 | 0.96916 | 1.04250 |
| | Submodel | Yes | 1.00001 | 0.96276 | 1.03378 |
| PALB2 | Full model | No | 1.06753 | 1.00419 | 1.13390 |
| | Full model | Yes | 1.06820 | 1.00483 | 1.13470 |
| PMS2 | Full model | No | 0.96191 | 0.91725 | 1.01165 |
| | Full model | Yes | 0.96116 | 0.91705 | 1.01091 |
| Any BM | Full model | No | 1.01611 | 0.99087 | 1.03973 |
| | Full model | Yes | 0.98866 | 0.96546 | 1.01159 |
| | Submodel | No | 1.01052 | 0.98470 | 1.03479 |
| | Submodel | Yes | 0.98464 | 0.96114 | 1.00807 |
| Any | Full model | No | 0.99695 | 0.98340 | 1.01193 |
| | Full model | Yes | 0.98903 | 0.97580 | 1.00354 |

Table S3: (continued from previous page)

(c) Mean squared error (MSE).

| Gene | Model | Risk Modifiers | Estimate | Bootstrap 2.5% | Bootstrap 97.5% |
|---|---|---|---|---|---|
| ATM | Full model | No | 0.00379 | 0.00367 | 0.00391 |
| | Full model | Yes | 0.00379 | 0.00367 | 0.00391 |
| BRCA1 | Full model | No | 0.00100 | 0.00095 | 0.00106 |
| | Full model | Yes | 0.00091 | 0.00086 | 0.00096 |
| | Submodel | No | 0.00101 | 0.00095 | 0.00106 |
| | Submodel | Yes | 0.00091 | 0.00086 | 0.00096 |
| BRCA2 | Full model | No | 0.00117 | 0.00111 | 0.00123 |
| | Full model | Yes | 0.00114 | 0.00109 | 0.00120 |
| | Submodel | No | 0.00117 | 0.00111 | 0.00124 |
| | Submodel | Yes | 0.00115 | 0.00109 | 0.00121 |
| BRCAPRO genes | Full model | No | 0.00203 | 0.00196 | 0.00211 |
| | Full model | Yes | 0.00199 | 0.00192 | 0.00206 |
| | Submodel | No | 0.00204 | 0.00197 | 0.00212 |
| | Submodel | Yes | 0.00200 | 0.00192 | 0.00207 |
| CDKN2A | Full model | No | 0.00029 | 0.00025 | 0.00032 |
| | Full model | Yes | 0.00029 | 0.00025 | 0.00032 |
| | Submodel | No | 0.00030 | 0.00027 | 0.00033 |
| | Submodel | Yes | 0.00030 | 0.00027 | 0.00033 |
| CHEK2 | Full model | No | 0.00530 | 0.00516 | 0.00543 |
| | Full model | Yes | 0.00530 | 0.00516 | 0.00543 |
| EPCAM | Full model | No | 0.00002 | 0.00001 | 0.00003 |
| | Full model | Yes | 0.00002 | 0.00001 | 0.00003 |
| MLH1 | Full model | No | 0.00068 | 0.00064 | 0.00073 |
| | Full model | Yes | 0.00064 | 0.00060 | 0.00068 |
| | Submodel | No | 0.00075 | 0.00070 | 0.00080 |
| | Submodel | Yes | 0.00069 | 0.00065 | 0.00073 |
| MSH2 | Full model | No | 0.00076 | 0.00071 | 0.00080 |
| | Full model | Yes | 0.00069 | 0.00065 | 0.00074 |
| | Submodel | No | 0.00083 | 0.00078 | 0.00088 |
| | Submodel | Yes | 0.00075 | 0.00071 | 0.00080 |
| MSH6 | Full model | No | 0.00032 | 0.00029 | 0.00035 |
| | Full model | Yes | 0.00031 | 0.00028 | 0.00035 |
| | Submodel | No | 0.00032 | 0.00029 | 0.00036 |
| | Submodel | Yes | 0.00032 | 0.00029 | 0.00035 |
| MMRpro genes | Full model | No | 0.00164 | 0.00158 | 0.00171 |
| | Full model | Yes | 0.00149 | 0.00143 | 0.00155 |
| | Submodel | No | 0.00176 | 0.00169 | 0.00183 |
| | Submodel | Yes | 0.00157 | 0.00151 | 0.00163 |
| PALB2 | Full model | No | 0.00106 | 0.00100 | 0.00113 |
| | Full model | Yes | 0.00106 | 0.00100 | 0.00113 |
| PMS2 | Full model | No | 0.00173 | 0.00165 | 0.00182 |
| | Full model | Yes | 0.00173 | 0.00164 | 0.00181 |
| Any BM | Full model | No | 0.00392 | 0.00383 | 0.00403 |
| | Full model | Yes | 0.00373 | 0.00363 | 0.00383 |
| | Submodel | No | 0.00406 | 0.00396 | 0.00417 |
| | Submodel | Yes | 0.00383 | 0.00373 | 0.00393 |
| Any | Full model | No | 0.01530 | 0.01506 | 0.01553 |
| | Full model | Yes | 0.01511 | 0.01488 | 0.01534 |

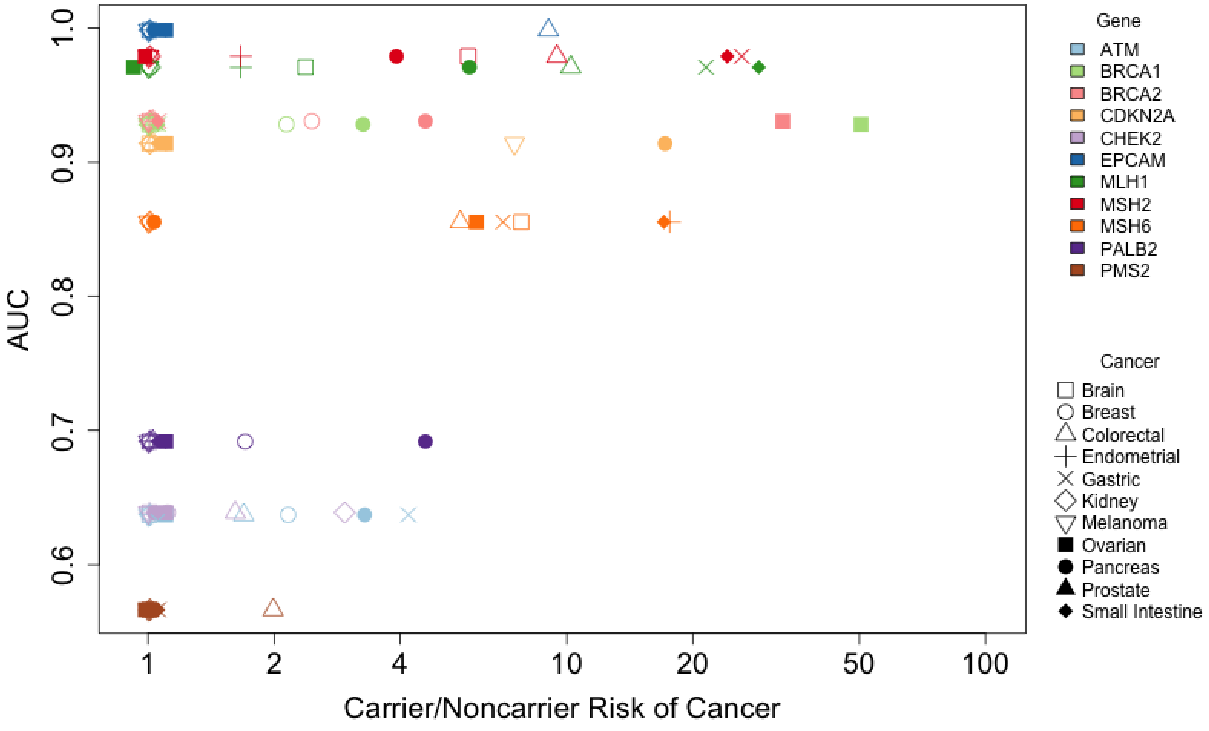


(a) Female relative risk at age 70.

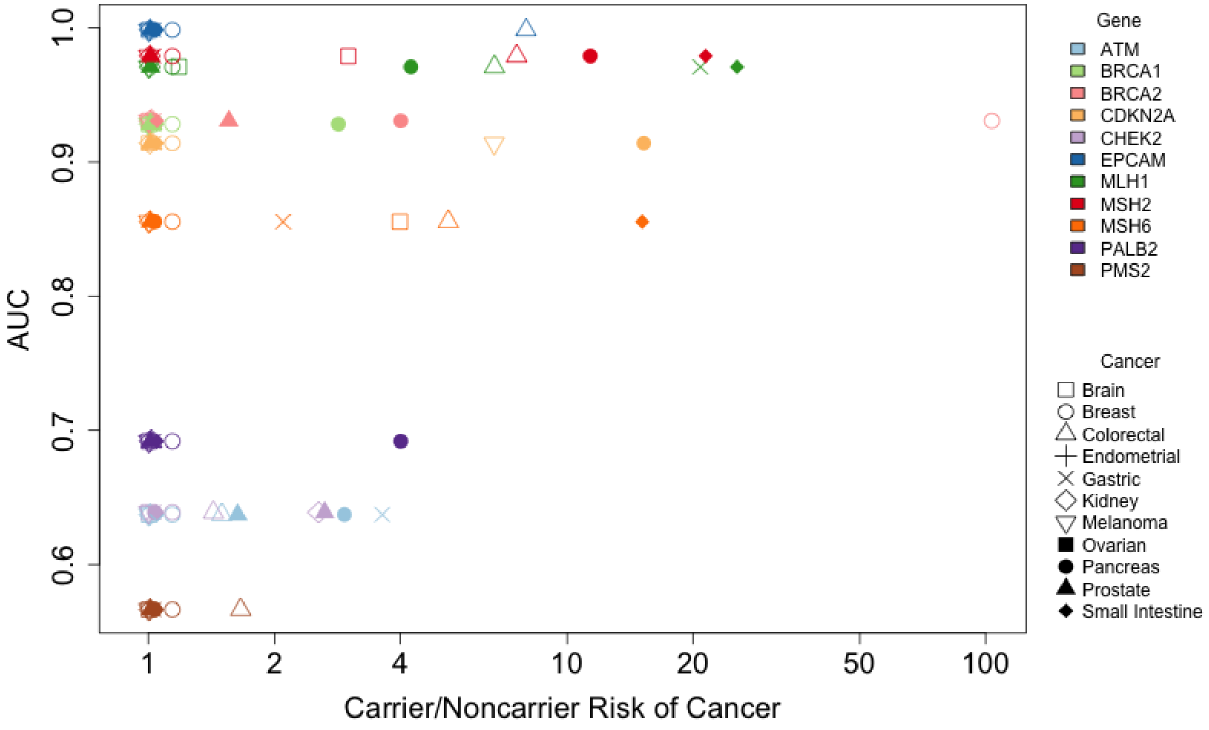


(b) Male relative risk at age 70.

Figure S2: Area under the curve (AUC) from evaluating PanelPRO-11 on 1,000,000 simulated families plotted against the relative risk of developing each cancer by age 70, for pathogenic variant carriers compared to noncarriers. Figure S2a shows the female relative risks only; Figure S2b shows the male relative risks only.

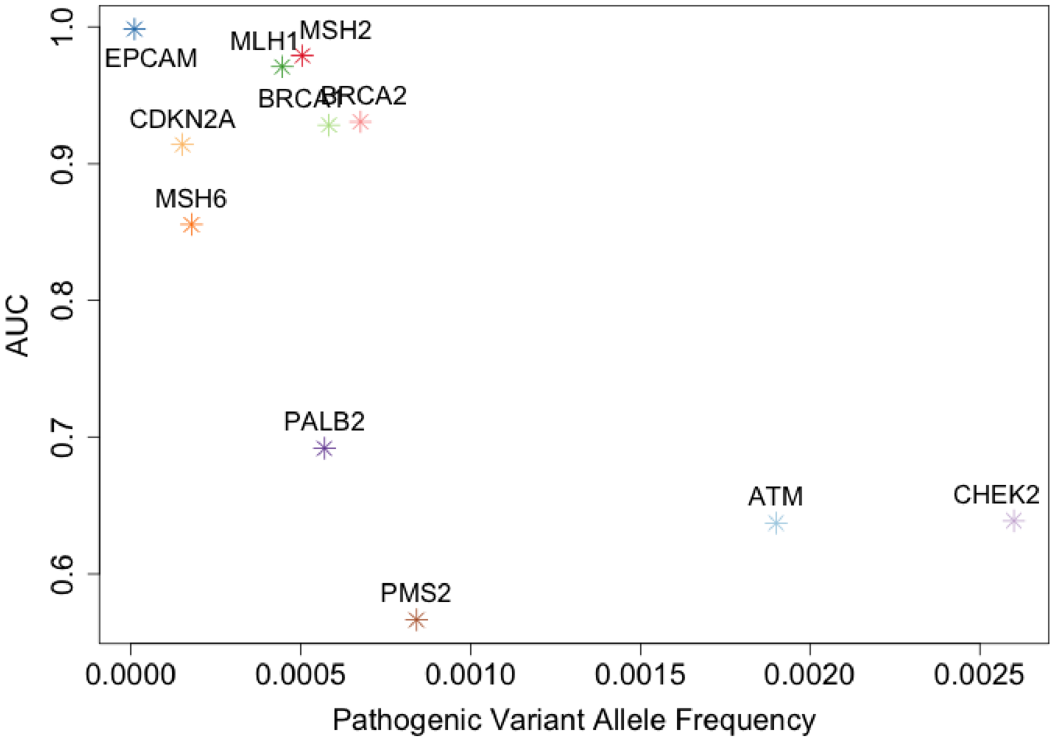


Figure S3: Area under the curve (AUC) from evaluating PanelPRO-11 on 1,000,000 simulated families plotted against allele frequency for pathogenic variants of each gene.

Table S4: Summary table of the area under the curve (AUC) for each gene from evaluating PanelPRO-11 on 1,000,000 simulated families; the population-level allele frequencies; and the male and female relative risks (RRs) of developing each cancer by age 70, for pathogenic variant carriers compared to noncarriers.

| | Sex | ATM | BRCA1 | BRCA2 | CDKN2A | CHEK2 | EPCAM |
|---|---|---|---|---|---|---|---|
| AUC | | 0.63715 | 0.92825 | 0.93066 | 0.91396 | 0.63884 | 0.99848 |
| Allele Frequency | | 0.00190 | 0.00058 | 0.00068 | 0.00015 | 0.00260 | 0.00001 |
| Brain RR (age 70) | Female | 1.00862 | 1.00862 | 1.00862 | 1.00862 | 1.00862 | 1.00862 |
| | Male | 1.00329 | 1.00329 | 1.00329 | 1.00329 | 1.00329 | 1.00329 |
| Breast RR (age 70) | Female | 2.15960 | 2.13913 | 2.45973 | 1.00913 | 1.11383 | 1.00913 |
| | Male | 1.15716 | 13.42021 | 104.94125 | 1.15716 | 1.15716 | 1.15716 |
| Colorectal RR (age 70) | Female | 1.69148 | 1.02613 | 1.02613 | 1.02613 | 1.61434 | 9.03956 |
| | Male | 1.49759 | 1.01867 | 1.01867 | 1.01867 | 1.42932 | 7.98353 |
| Endometrial RR (age 70) | Female | 1.00729 | 1.00729 | 1.00729 | 1.00729 | 1.00729 | 1.00729 |
| Gastric RR (age 70) | Female | 4.18469 | 1.05851 | 1.05851 | 1.05851 | 1.05851 | 1.05851 |
| | Male | 3.61984 | 1.02830 | 1.02830 | 1.02830 | 1.02830 | 1.02830 |
| Kidney RR (age 70) | Female | 1.01022 | 1.01022 | 1.01022 | 1.01022 | 2.94692 | 1.01022 |
| | Male | 1.00813 | 1.00813 | 1.00813 | 1.00813 | 2.54899 | 1.00813 |
| Melanoma RR (age 70) | Female | 1.00201 | 1.00201 | 1.00201 | 7.49881 | 1.00201 | 1.00201 |
| | Male | 1.00176 | 1.00176 | 1.00176 | 6.69797 | 1.00176 | 1.00176 |
| Ovarian RR (age 70) | Female | 1.13082 | 51.71606 | 51.71606 | 1.13082 | 1.13082 | 1.13082 |
| Pancreas RR (age 70) | Female | 3.28904 | 3.26071 | 4.59356 | 17.16520 | 1.03267 | 1.03267 |
| | Male | 2.93797 | 2.84351 | 4.00583 | 15.25511 | 1.03490 | 1.03490 |
| Prostate RR (age 70) | Male | 1.63399 | 1.01172 | 1.55695 | 1.01172 | 2.63701 | 1.01172 |
| Small Intestine RR (age 70) | Female | 1.05460 | 1.05460 | 1.05460 | 1.05460 | 1.05460 | 1.05460 |
| | Male | 1.04813 | 1.04813 | 1.04813 | 1.04813 | 1.04813 | 1.04813 |

| | Sex | MLH1 | MSH2 | MSH6 | PALB2 | PMS2 |
|---|---|---|---|---|---|---|
| AUC | | 0.97091 | 0.97901 | 0.85549 | 0.69181 | 0.56632 |
| Allele Frequency | | 0.00045 | 0.00050 | 0.00018 | 0.00057 | 0.00084 |
| Brain RR (age 70) | Female | 2.37521 | 5.81166 | 7.78749 | 1.00862 | 1.00862 |
| | Male | 1.18235 | 3.00266 | 3.98669 | 1.00329 | 1.00329 |
| Breast RR (age 70) | Female | 1.00913 | 1.00913 | 1.00913 | 1.70461 | 1.00913 |
| | Male | 1.15716 | 1.15716 | 1.15716 | 1.15716 | 1.15716 |
| Colorectal RR (age 70) | Female | 10.22819 | 9.47057 | 5.56418 | 1.02613 | 1.98866 |
| | Male | 6.70954 | 7.57958 | 5.20577 | 1.01867 | 1.66110 |
| Endometrial RR (age 70) | Female | 1.66514 | 1.66514 | 17.61259 | 1.00729 | 1.00729 |
| Gastric RR (age 70) | Female | 21.49716 | 26.17219 | 7.04253 | 1.05851 | 1.05851 |
| | Male | 20.81028 | 1.02830 | 2.09849 | 1.02830 | 1.02830 |
| Kidney RR (age 70) | Female | 1.01022 | 1.01022 | 1.01022 | 1.01022 | 1.01022 |
| | Male | 1.00813 | 1.00813 | 1.00813 | 1.00813 | 1.00813 |
| Melanoma RR (age 70) | Female | 1.00201 | 1.00201 | 1.00201 | 1.00201 | 1.00201 |
| | Male | 1.00176 | 1.00176 | 1.00176 | 1.00176 | 1.00176 |
| Ovarian RR (age 70) | Female | 0.94605 | 1.00832 | 6.23502 | 1.13082 | 1.00832 |
| Pancreas RR (age 70) | Female | 5.85305 | 3.91862 | 1.03267 | 4.59356 | 1.03267 |
| | Male | 4.23564 | 11.36407 | 1.03490 | 4.00583 | 1.03490 |
| Prostate RR (age 70) | Male | 1.01172 | 1.01172 | 1.01172 | 1.01172 | 1.01172 |
| Small Intestine RR (age 70) | Female | 28.75099 | 24.16518 | 17.06113 | 1.05460 | 1.05460 |
| | Male | 25.48554 | 21.42057 | 15.12337 | 1.04813 | 1.04813 |

## S4 PanelPRO-11 Simulations with PRSs

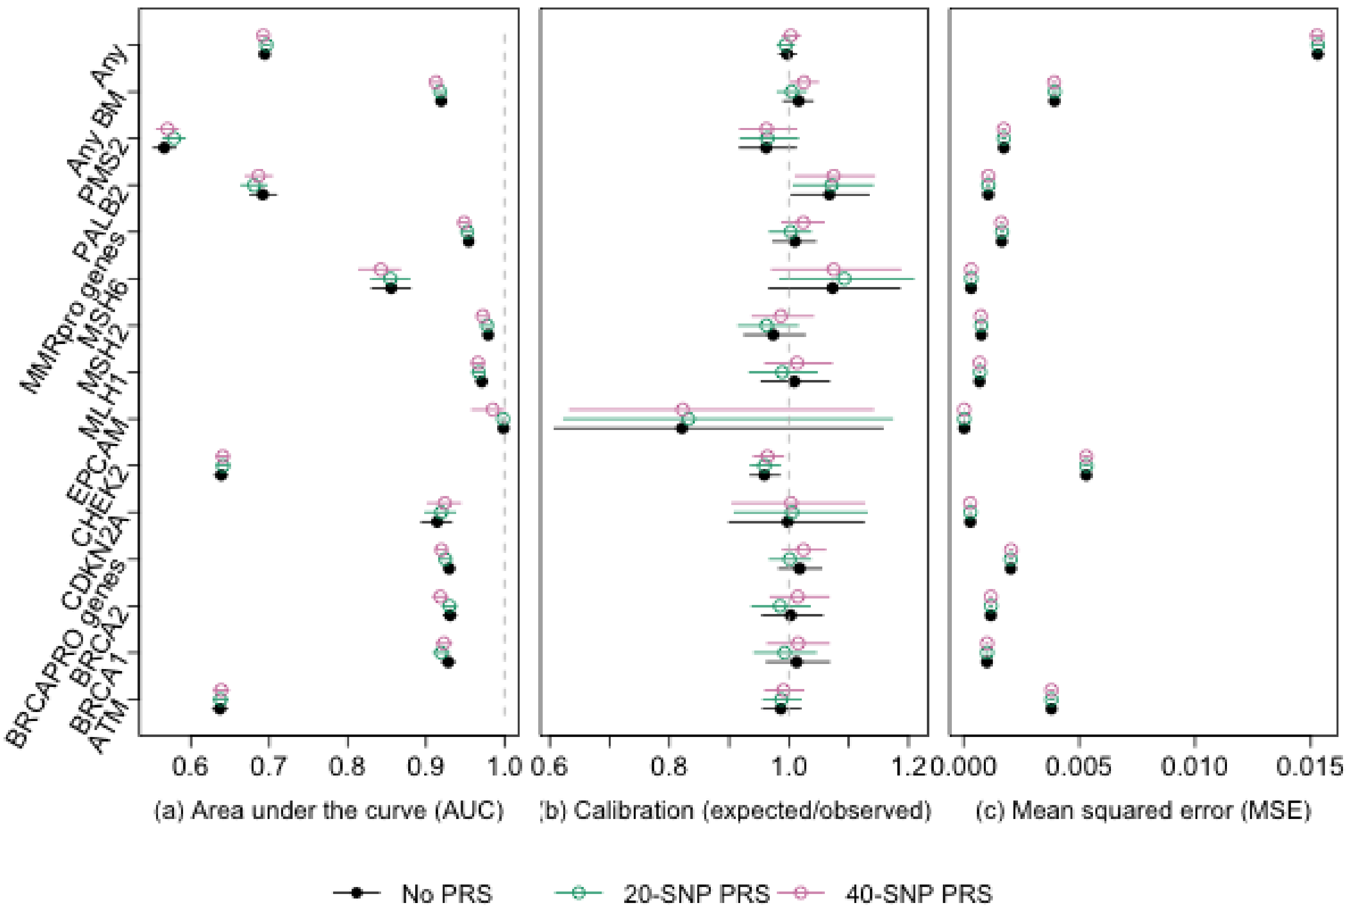


Figure S4: AUC, calibration, and MSE for PanelPRO-11 evaluated on 1,000,000 families simulated based on PanelPRO-11 (black solid points), PanelPRO-11 with a 20-SNP (green open points), and PanelPRO-11 with 40-SNP PRS (purple open points). All families were simulated without additional risk modifiers. "BRCAPRO genes", "MMRpro genes", and "Any BM" indicate any of the genes in BRCAPRO (BRCA1, BRCA2), MMRpro (MLH1, MSH2, MSH6), and any model in the BayesMendel package (BRCA1, BRCA2, MLH1, MSH2, MSH6, CDKN2A), respectively. "Any" indicates any of the eleven genes in PanelPRO-11. 95% bootstrap percentile confidence intervals are also shown.

Table S5: AUC, calibration, and MSE for PanelPRO-11 evaluated on 1,000,000 families simulated based on PanelPRO-11, PanelPRO-11 with a 20-SNP, and PanelPRO-11 with 40-SNP PRS. All families were simulated without additional risk modifiers. "BRCAPRO genes", "MMRpro genes", and "Any BM" indicate any of the genes in BRCAPRO (BRCA1, BRCA2), MMRpro (MLH1, MSH2, MSH6), and any model in the BayesMendel package (BRCA1, BRCA2, MLH1, MSH2, MSH6, CDKN2A), respectively. "Any" indicates any of the eleven genes in PanelPRO-11. 95% bootstrap percentile confidence intervals are also shown.

(a) Area under the curve (AUC).

| Gene | Data | Estimate | Bootstrap 2.5% | Bootstrap 97.5% |
|---|---|---|---|---|
| ATM | No PRS | 0.63715 | 0.62847 | 0.64688 |
| | 20-SNP PRS | 0.63804 | 0.62961 | 0.64745 |
| | 40-SNP PRS | 0.63887 | 0.63021 | 0.64828 |
| BRCA1 | No PRS | 0.92825 | 0.91939 | 0.93722 |
| | 20-SNP PRS | 0.91917 | 0.90930 | 0.92926 |
| | 40-SNP PRS | 0.92261 | 0.91328 | 0.93227 |
| BRCA2 | No PRS | 0.93066 | 0.92211 | 0.93809 |
| | 20-SNP PRS | 0.92978 | 0.92062 | 0.93803 |
| | 40-SNP PRS | 0.91790 | 0.90856 | 0.92721 |
| BRCAPRO genes | No PRS | 0.92943 | 0.92318 | 0.93547 |
| | 20-SNP PRS | 0.92442 | 0.91719 | 0.93141 |
| | 40-SNP PRS | 0.91942 | 0.91266 | 0.92567 |
| CDKN2A | No PRS | 0.91396 | 0.89417 | 0.93228 |
| | 20-SNP PRS | 0.91908 | 0.89898 | 0.93717 |
| | 40-SNP PRS | 0.92365 | 0.90192 | 0.94378 |
| CHEK2 | No PRS | 0.63884 | 0.63051 | 0.64687 |
| | 20-SNP PRS | 0.64115 | 0.63348 | 0.64859 |
| | 40-SNP PRS | 0.64091 | 0.63316 | 0.64818 |
| EPCAM | No PRS | 0.99848 | 0.99712 | 0.99958 |
| | 20-SNP PRS | 0.99819 | 0.99502 | 0.99993 |
| | 40-SNP PRS | 0.98500 | 0.95840 | 0.99990 |
| MLH1 | No PRS | 0.97091 | 0.96442 | 0.97703 |
| | 20-SNP PRS | 0.96696 | 0.95908 | 0.97384 |
| | 40-SNP PRS | 0.96609 | 0.95850 | 0.97299 |
| MSH2 | No PRS | 0.97901 | 0.97384 | 0.98374 |
| | 20-SNP PRS | 0.97773 | 0.97190 | 0.98273 |
| | 40-SNP PRS | 0.97219 | 0.96575 | 0.97806 |
| MSH6 | No PRS | 0.85549 | 0.83085 | 0.87974 |
| | 20-SNP PRS | 0.85445 | 0.82982 | 0.87896 |
| | 40-SNP PRS | 0.84224 | 0.81461 | 0.86693 |
| MMRpro genes | No PRS | 0.95419 | 0.94836 | 0.95928 |
| | 20-SNP PRS | 0.95254 | 0.94619 | 0.95743 |
| | 40-SNP PRS | 0.94831 | 0.94201 | 0.95383 |
| PALB2 | No PRS | 0.69181 | 0.67586 | 0.70905 |
| | 20-SNP PRS | 0.68074 | 0.66437 | 0.69686 |
| | 40-SNP PRS | 0.68641 | 0.66997 | 0.70367 |
| PMS2 | No PRS | 0.56632 | 0.55240 | 0.58072 |
| | 20-SNP PRS | 0.57871 | 0.56489 | 0.59264 |
| | 40-SNP PRS | 0.57057 | 0.55643 | 0.58427 |
| Any BM | No PRS | 0.91916 | 0.91422 | 0.92370 |
| | 20-SNP PRS | 0.91761 | 0.91268 | 0.92231 |
| | 40-SNP PRS | 0.91244 | 0.90733 | 0.91729 |
| Any | No PRS | 0.69430 | 0.69034 | 0.69909 |
| | 20-SNP PRS | 0.69662 | 0.69215 | 0.70092 |
| | 40-SNP PRS | 0.69241 | 0.68787 | 0.69717 |

Table S5: (continued from previous page)

(b) Calibration (expected divided by observed number of events).

| Gene | Data | Estimate | Bootstrap 2.5% | Bootstrap 97.5% |
|---|---|---|---|---|
| ATM | No PRS | 0.98627 | 0.95630 | 1.01938 |
| | 20-SNP PRS | 0.98706 | 0.95701 | 1.01997 |
| | 40-SNP PRS | 0.99078 | 0.96014 | 1.02397 |
| BRCA1 | No PRS | 1.01273 | 0.96276 | 1.06748 |
| | 20-SNP PRS | 0.99262 | 0.94186 | 1.04525 |
| | 40-SNP PRS | 1.01543 | 0.96410 | 1.06656 |
| BRCA2 | No PRS | 1.00296 | 0.95526 | 1.05576 |
| | 20-SNP PRS | 0.98484 | 0.93810 | 1.03513 |
| | 40-SNP PRS | 1.01464 | 0.96928 | 1.06622 |
| BRCAPRO genes | No PRS | 1.01781 | 0.98310 | 1.05425 |
| | 20-SNP PRS | 1.00132 | 0.96766 | 1.03607 |
| | 40-SNP PRS | 1.02422 | 0.98938 | 1.06110 |
| CDKN2A | No PRS | 0.99774 | 0.89985 | 1.12565 |
| | 20-SNP PRS | 1.00494 | 0.90864 | 1.13035 |
| | 40-SNP PRS | 1.00355 | 0.90519 | 1.12630 |
| CHEK2 | No PRS | 0.95887 | 0.93569 | 0.98478 |
| | 20-SNP PRS | 0.95926 | 0.93606 | 0.98518 |
| | 40-SNP PRS | 0.96402 | 0.94087 | 0.99035 |
| EPCAM | No PRS | 0.82103 | 0.60819 | 1.15672 |
| | 20-SNP PRS | 0.83200 | 0.62329 | 1.17286 |
| | 40-SNP PRS | 0.82233 | 0.63391 | 1.14072 |
| MLH1 | No PRS | 1.00885 | 0.95408 | 1.06722 |
| | 20-SNP PRS | 0.98844 | 0.93444 | 1.04682 |
| | 40-SNP PRS | 1.01338 | 0.96022 | 1.07150 |
| MSH2 | No PRS | 0.97349 | 0.92525 | 1.02685 |
| | 20-SNP PRS | 0.96246 | 0.91539 | 1.01470 |
| | 40-SNP PRS | 0.98618 | 0.93886 | 1.04066 |
| MSH6 | No PRS | 1.07297 | 0.96656 | 1.18515 |
| | 20-SNP PRS | 1.09255 | 0.98448 | 1.20846 |
| | 40-SNP PRS | 1.07463 | 0.97131 | 1.18664 |
| MMRpro genes | No PRS | 1.00979 | 0.97323 | 1.04471 |
| | 20-SNP PRS | 1.00294 | 0.96744 | 1.03659 |
| | 40-SNP PRS | 1.02384 | 0.98843 | 1.05804 |
| PALB2 | No PRS | 1.06753 | 1.00419 | 1.13390 |
| | 20-SNP PRS | 1.07095 | 1.00760 | 1.14020 |
| | 40-SNP PRS | 1.07464 | 1.01157 | 1.14244 |
| PMS2 | No PRS | 0.96191 | 0.91725 | 1.01165 |
| | 20-SNP PRS | 0.96363 | 0.91905 | 1.01477 |
| | 40-SNP PRS | 0.96243 | 0.91783 | 1.01230 |
| Any BM | No PRS | 1.01611 | 0.99087 | 1.03973 |
| | 20-SNP PRS | 1.00452 | 0.98075 | 1.02850 |
| | 40-SNP PRS | 1.02495 | 1.00161 | 1.04915 |
| Any | No PRS | 0.99695 | 0.98340 | 1.01193 |
| | 20-SNP PRS | 0.99411 | 0.98068 | 1.00934 |
| | 40-SNP PRS | 1.00291 | 0.98903 | 1.01829 |

Table S5: (continued from previous page)

(c) Mean squared error (MSE).

| Gene | Data | Estimate | Bootstrap 2.5% | Bootstrap 97.5% |
|---|---|---|---|---|
| ATM | No PRS | 0.00379 | 0.00367 | 0.00391 |
| | 20-SNP PRS | 0.00379 | 0.00367 | 0.00391 |
| | 40-SNP PRS | 0.00379 | 0.00367 | 0.00391 |
| BRCA1 | No PRS | 0.00100 | 0.00095 | 0.00106 |
| | 20-SNP PRS | 0.00100 | 0.00095 | 0.00106 |
| | 40-SNP PRS | 0.00101 | 0.00095 | 0.00106 |
| BRCA2 | No PRS | 0.00117 | 0.00111 | 0.00123 |
| | 20-SNP PRS | 0.00117 | 0.00111 | 0.00123 |
| | 40-SNP PRS | 0.00117 | 0.00111 | 0.00123 |
| BRCAPRO genes | No PRS | 0.00203 | 0.00196 | 0.00211 |
| | 20-SNP PRS | 0.00203 | 0.00196 | 0.00211 |
| | 40-SNP PRS | 0.00205 | 0.00197 | 0.00212 |
| CDKN2A | No PRS | 0.00029 | 0.00025 | 0.00032 |
| | 20-SNP PRS | 0.00029 | 0.00025 | 0.00032 |
| | 40-SNP PRS | 0.00028 | 0.00025 | 0.00031 |
| CHEK2 | No PRS | 0.00530 | 0.00516 | 0.00543 |
| | 20-SNP PRS | 0.00530 | 0.00516 | 0.00543 |
| | 40-SNP PRS | 0.00530 | 0.00516 | 0.00543 |
| EPCAM | No PRS | 0.00002 | 0.00001 | 0.00003 |
| | 20-SNP PRS | 0.00002 | 0.00001 | 0.00003 |
| | 40-SNP PRS | 0.00002 | 0.00001 | 0.00003 |
| MLH1 | No PRS | 0.00068 | 0.00064 | 0.00073 |
| | 20-SNP PRS | 0.00070 | 0.00066 | 0.00075 |
| | 40-SNP PRS | 0.00069 | 0.00065 | 0.00073 |
| MSH2 | No PRS | 0.00076 | 0.00071 | 0.00080 |
| | 20-SNP PRS | 0.00075 | 0.00071 | 0.00080 |
| | 40-SNP PRS | 0.00074 | 0.00069 | 0.00078 |
| MSH6 | No PRS | 0.00032 | 0.00029 | 0.00035 |
| | 20-SNP PRS | 0.00032 | 0.00029 | 0.00035 |
| | 40-SNP PRS | 0.00032 | 0.00029 | 0.00035 |
| MMRpro genes | No PRS | 0.00164 | 0.00158 | 0.00171 |
| | 20-SNP PRS | 0.00165 | 0.00159 | 0.00172 |
| | 40-SNP PRS | 0.00162 | 0.00156 | 0.00169 |
| PALB2 | No PRS | 0.00106 | 0.00100 | 0.00113 |
| | 20-SNP PRS | 0.00106 | 0.00100 | 0.00113 |
| | 40-SNP PRS | 0.00106 | 0.00100 | 0.00113 |
| PMS2 | No PRS | 0.00173 | 0.00165 | 0.00182 |
| | 20-SNP PRS | 0.00173 | 0.00165 | 0.00182 |
| | 40-SNP PRS | 0.00173 | 0.00165 | 0.00182 |
| Any BM | No PRS | 0.00392 | 0.00383 | 0.00403 |
| | 20-SNP PRS | 0.00393 | 0.00383 | 0.00404 |
| | 40-SNP PRS | 0.00391 | 0.00381 | 0.00401 |
| Any | No PRS | 0.01530 | 0.01506 | 0.01553 |
| | 20-SNP PRS | 0.01531 | 0.01507 | 0.01553 |
| | 40-SNP PRS | 0.01527 | 0.01504 | 0.01549 |

# S5 PanelPRO-5BC Validation on HCP Cohort

Table S6: AUC, calibration, and MSE for the full PanelPRO-5BC model and its BRCAPRO submodel evaluated on the HCP cohort, with and without risk modifiers. “BRCAPRO genes” indicates any of the genes in BRCAPRO (BRCA1, BRCA2), and “Any” indicates any of the five genes in PanelPRO-5BC. 95% bootstrap percentile confidence intervals are also reported.

(a) Area under the curve (AUC).

| Gene | Model | Risk Modifiers | Estimate | Bootstrap 2.5% | Bootstrap 97.5% |
|---|---|---|---|---|---|
| ATM | Full model | No | 0.61944 | 0.47854 | 0.78247 |
| | Full model | Yes | 0.61867 | 0.47449 | 0.78506 |
| BRCA1 | Full model | No | 0.82502 | 0.75408 | 0.88664 |
| | Full model | Yes | 0.78735 | 0.70806 | 0.86267 |
| | Submodel | No | 0.82470 | 0.75410 | 0.88629 |
| | Submodel | Yes | 0.78709 | 0.70798 | 0.86259 |
| BRCA2 | Full model | No | 0.67855 | 0.58382 | 0.75894 |
| | Full model | Yes | 0.69755 | 0.60496 | 0.77873 |
| | Submodel | No | 0.67881 | 0.58397 | 0.75881 |
| | Submodel | Yes | 0.69749 | 0.60515 | 0.77905 |
| BRCAPRO genes | Full model | No | 0.75616 | 0.69464 | 0.80701 |
| | Full model | Yes | 0.75682 | 0.69589 | 0.81229 |
| | Submodel | No | 0.75600 | 0.69403 | 0.80639 |
| | Submodel | Yes | 0.75682 | 0.69538 | 0.81211 |
| CHEK2 | Full model | No | 0.48791 | 0.43141 | 0.68304 |
| | Full model | Yes | 0.52160 | 0.44753 | 0.68668 |
| PALB2 | Full model | No | 0.63279 | 0.48168 | 0.83771 |
| | Full model | Yes | 0.64584 | 0.47912 | 0.85189 |
| Any | Full model | No | 0.67436 | 0.61491 | 0.72804 |
| | Full model | Yes | 0.67695 | 0.61764 | 0.73057 |

(b) Calibration (expected divided by observed number of events).

| Gene | Model | Risk Modifiers | Estimate | Bootstrap 2.5% | Bootstrap 97.5% |
|---|---|---|---|---|---|
| ATM | Full model | No | 1.17429 | 0.68925 | 2.43607 |
| | Full model | Yes | 1.09484 | 0.63547 | 2.26672 |
| BRCA1 | Full model | No | 0.73783 | 0.53406 | 1.04564 |
| | Full model | Yes | 1.85462 | 1.41912 | 2.58837 |
| | Submodel | No | 0.75885 | 0.54988 | 1.06914 |
| | Submodel | Yes | 1.86138 | 1.42286 | 2.59631 |
| BRCA2 | Full model | No | 0.80527 | 0.56862 | 1.21781 |
| | Full model | Yes | 0.71557 | 0.49557 | 1.08699 |
| | Submodel | No | 0.83172 | 0.58883 | 1.26896 |
| | Submodel | Yes | 0.72816 | 0.50397 | 1.10827 |
| BRCAPRO genes | Full model | No | 0.67139 | 0.53990 | 0.86996 |
| | Full model | Yes | 1.23301 | 1.00652 | 1.56922 |
| | Submodel | No | 0.68329 | 0.54760 | 0.87967 |
| | Submodel | Yes | 1.23177 | 1.00590 | 1.56028 |
| CHEK2 | Full model | No | 1.11064 | 0.70807 | 2.18568 |
| | Full model | Yes | 1.05207 | 0.66774 | 2.06927 |
| PALB2 | Full model | No | 1.14825 | 0.56474 | 3.01631 |
| | Full model | Yes | 0.98453 | 0.46672 | 2.76324 |
| Any | Full model | No | 0.70763 | 0.58871 | 0.86623 |
| | Full model | Yes | 1.04282 | 0.87473 | 1.27218 |

Table S6: (continued from previous page)

(c) Mean squared error (MSE).

| Gene | Model | Risk Modifiers | Estimate | Bootstrap 2.5% | Bootstrap 97.5% |
|---|---|---|---|---|---|
| ATM | Full model | No | 0.01126 | 0.00617 | 0.01642 |
| | Full model | Yes | 0.01121 | 0.00616 | 0.01638 |
| BRCA1 | Full model | No | 0.02653 | 0.01930 | 0.03443 |
| | Full model | Yes | 0.03643 | 0.02879 | 0.04417 |
| | Submodel | No | 0.02677 | 0.01948 | 0.03457 |
| | Submodel | Yes | 0.03655 | 0.02892 | 0.04428 |
| BRCA2 | Full model | No | 0.02779 | 0.02014 | 0.03561 |
| | Full model | Yes | 0.02733 | 0.01953 | 0.03512 |
| | Submodel | No | 0.02799 | 0.02032 | 0.03584 |
| | Submodel | Yes | 0.02749 | 0.01967 | 0.03524 |
| BRCAPRO genes | Full model | No | 0.04787 | 0.03839 | 0.05735 |
| | Full model | Yes | 0.05477 | 0.04513 | 0.06447 |
| | Submodel | No | 0.04824 | 0.03889 | 0.05773 |
| | Submodel | Yes | 0.05487 | 0.04522 | 0.06449 |
| CHEK2 | Full model | No | 0.01337 | 0.00810 | 0.01871 |
| | Full model | Yes | 0.01332 | 0.00807 | 0.01869 |
| PALB2 | Full model | No | 0.00868 | 0.00459 | 0.01390 |
| | Full model | Yes | 0.00866 | 0.00464 | 0.01393 |
| Any | Full model | No | 0.06876 | 0.05784 | 0.07980 |
| | Full model | Yes | 0.07505 | 0.06404 | 0.08632 |

# S6 PanelPRO-11 Validation on HCP Cohort

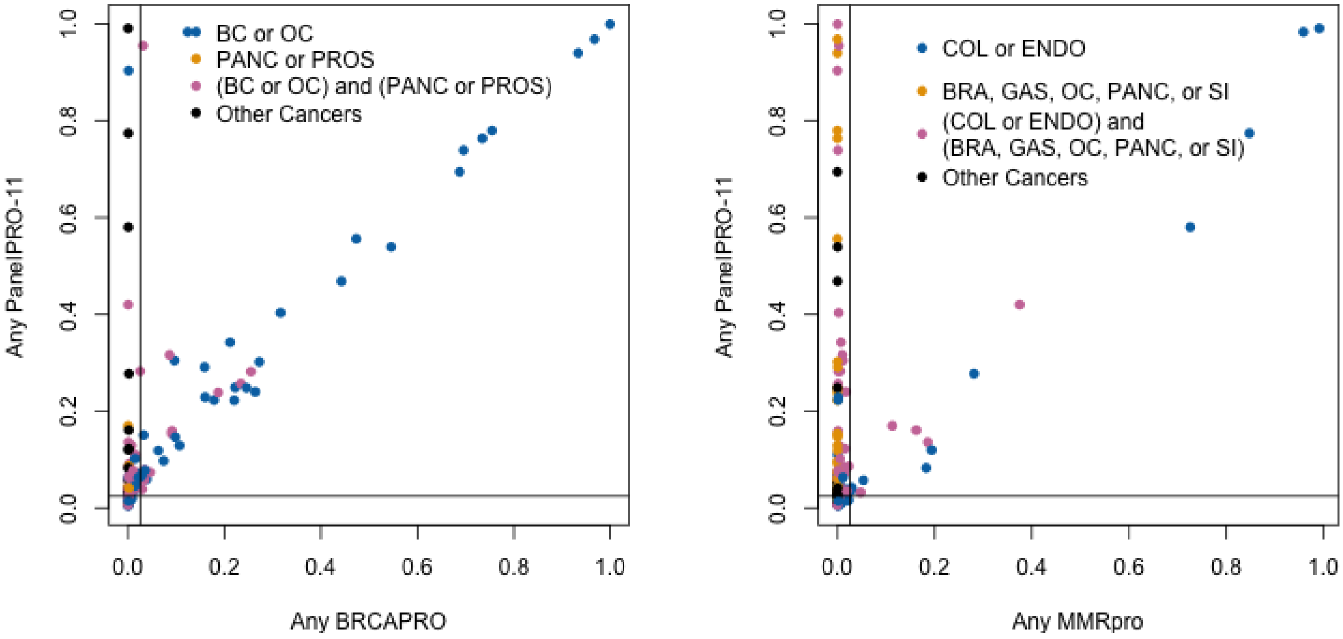


Figure S5: Probabilities of carrying a pathogenic variant of any PanelPRO-11 gene plotted against the probabilities for carrying a pathogenic variant of any BRCAPRO gene (BRCA1 or BRCA2, left) and against the probabilities for carrying a pathogenic variant of any MMRpro gene (MLH1, MSH2, or MSH6, right) in the HCP cohort. All counselees shown are true pathogenic variant carriers. The points are colored based on the cancer types represented in the counselee's family history. Counselees with family history of cancers incorporated in each syndrome-specific model (breast and ovarian cancer for BRCAPRO; colorectal and endometrial cancer for MMRpro) are colored blue. Those with family history of additional cancers associated with the syndrome-specific model's genes are colored orange (pancreatic and prostate cancer are also associated with BRCA1 and BRCA2; brain, gastric, ovarian, pancreatic, and small intestine cancer are other Lynch syndrome cancers). Counselees with family history of both of these groups of cancers (both cancers that are incorporated in the given syndrome-specific model and relevant cancers that are not) are colored purple. Reference lines are drawn at 2.5%.

Table S7: AUC, calibration, and MSE for the full PanelPRO-11 model and its BayesMendel submodels BRCAPRO, MMRpro, and Melapro evaluated on the HCP cohort, with and without risk modifiers. “BRCAPRO genes”, “MMRpro genes”, and “Any BM” indicate any of the genes in BRCAPRO (BRCA1, BRCA2), MMRpro (MLH1, MSH2, MSH6), and any model in the BayesMendel package (BRCA1, BRCA2, MLH1, MSH2, MSH6, CDKN2A), respectively. “Any” indicates any of the eleven genes in PanelPRO-11. 95% bootstrap percentile confidence intervals are also reported.

(a) Area under the curve (AUC).

| Gene | Model | Risk Modifiers | Estimate | Bootstrap 2.5% | Bootstrap 97.5% |
|---|---|---|---|---|---|
| ATM | Full model | No | 0.59478 | 0.47680 | 0.76613 |
| | Full model | Yes | 0.58895 | 0.45033 | 0.76434 |
| BRCA1 | Full model | No | 0.82414 | 0.75479 | 0.88541 |
| | Full model | Yes | 0.78554 | 0.70478 | 0.85861 |
| | Submodel | No | 0.82185 | 0.75137 | 0.88426 |
| | Submodel | Yes | 0.78493 | 0.70428 | 0.85728 |
| BRCA2 | Full model | No | 0.66842 | 0.56442 | 0.76003 |
| | Full model | Yes | 0.68563 | 0.58106 | 0.77571 |
| | Submodel | No | 0.67431 | 0.58107 | 0.76329 |
| | Submodel | Yes | 0.69295 | 0.60033 | 0.78106 |
| BRCAPRO genes | Full model | No | 0.75229 | 0.68726 | 0.80875 |
| | Full model | Yes | 0.75111 | 0.68660 | 0.80914 |
| | Submodel | No | 0.75225 | 0.69046 | 0.80648 |
| | Submodel | Yes | 0.75396 | 0.69234 | 0.81299 |
| CDKN2A | Full model | No | 0.98558 | 0.97939 | 0.99177 |
| | Full model | Yes | 0.98710 | 0.98100 | 0.99320 |
| | Submodel | No | 0.99393 | 0.98934 | 0.99773 |
| | Submodel | Yes | 0.99393 | 0.98934 | 0.99773 |
| CHEK2 | Full model | No | 0.48543 | 0.44348 | 0.66200 |
| | Full model | Yes | 0.52721 | 0.44780 | 0.66644 |
| EPCAM | Full model | No | 0.99697 | 0.99394 | 0.99957 |
| | Full model | Yes | 0.99697 | 0.99394 | 0.99957 |
| MLH1 | Full model | No | 0.94470 | 0.89722 | 0.97960 |
| | Full model | Yes | 0.94596 | 0.89938 | 0.98082 |
| | Submodel | No | 0.96206 | 0.92667 | 0.98936 |
| | Submodel | Yes | 0.96232 | 0.92638 | 0.98973 |
| MSH2 | Full model | No | 0.83881 | 0.73263 | 0.92378 |
| | Full model | Yes | 0.85184 | 0.73683 | 0.93779 |
| | Submodel | No | 0.85598 | 0.76487 | 0.93622 |
| | Submodel | Yes | 0.86543 | 0.76868 | 0.94785 |
| MSH6 | Full model | No | 0.68448 | 0.51526 | 0.84725 |
| | Full model | Yes | 0.68675 | 0.51768 | 0.84854 |
| | Submodel | No | 0.75645 | 0.57875 | 0.89013 |
| | Submodel | Yes | 0.75634 | 0.58039 | 0.88872 |
| MMRpro genes | Full model | No | 0.80692 | 0.71909 | 0.87900 |
| | Full model | Yes | 0.81223 | 0.72553 | 0.88591 |
| | Submodel | No | 0.85312 | 0.78226 | 0.91150 |
| | Submodel | Yes | 0.85758 | 0.78688 | 0.91675 |
| PALB2 | Full model | No | 0.60613 | 0.46485 | 0.84361 |
| | Full model | Yes | 0.61675 | 0.46885 | 0.85339 |
| PMS2 | Full model | No | 0.51035 | 0.46136 | 0.71145 |
| | Full model | Yes | 0.51966 | 0.46866 | 0.71568 |
| Any BM | Full model | No | 0.69701 | 0.64183 | 0.75275 |
| | Full model | Yes | 0.69895 | 0.64344 | 0.75402 |
| | Submodel | No | 0.69003 | 0.63255 | 0.74458 |
| | Submodel | Yes | 0.69711 | 0.63987 | 0.75186 |
| Any | Full model | No | 0.64489 | 0.59798 | 0.69337 |
| | Full model | Yes | 0.64405 | 0.59691 | 0.69615 |

Table S7: (continued from previous page)

(b) Calibration (expected divided by observed number of events).

| Gene | Model | Risk Modifiers | Estimate | Bootstrap 2.5% | Bootstrap 97.5% |
|---|---|---|---|---|---|
| ATM | Full model | No | 1.20604 | 0.74641 | 2.64397 |
| | Full model | Yes | 1.12886 | 0.69061 | 2.46664 |
| BRCA1 | Full model | No | 0.66618 | 0.49216 | 0.93316 |
| | Full model | Yes | 1.63567 | 1.22956 | 2.23680 |
| | Submodel | No | 0.68963 | 0.51346 | 0.97366 |
| | Submodel | Yes | 1.64041 | 1.23296 | 2.24257 |
| BRCA2 | Full model | No | 0.70521 | 0.47346 | 1.08308 |
| | Full model | Yes | 0.63838 | 0.41710 | 0.97448 |
| | Submodel | No | 0.74140 | 0.50279 | 1.13024 |
| | Submodel | Yes | 0.65297 | 0.43575 | 1.00560 |
| BRCAPRO genes | Full model | No | 0.61319 | 0.47020 | 0.78285 |
| | Full model | Yes | 1.11184 | 0.88849 | 1.40041 |
| | Submodel | No | 0.62390 | 0.47926 | 0.80069 |
| | Submodel | Yes | 1.10004 | 0.87661 | 1.38576 |
| CDKN2A | Full model | No | 7.81779 | 1.66689 | 7.81779 |
| | Full model | Yes | 7.71707 | 1.64669 | 7.71707 |
| | Submodel | No | 4.36598 | 1.05478 | 4.36598 |
| | Submodel | Yes | 4.36598 | 1.05478 | 4.36598 |
| CHEK2 | Full model | No | 1.05752 | 0.64159 | 2.07377 |
| | Full model | Yes | 1.01043 | 0.61059 | 1.97048 |
| EPCAM | Full model | No | 3.57143 | 0.42806 | 3.57143 |
| | Full model | Yes | 3.57097 | 0.42792 | 3.57097 |
| MLH1 | Full model | No | 1.61178 | 0.89169 | 4.00383 |
| | Full model | Yes | 1.65814 | 0.95915 | 4.02794 |
| | Submodel | No | 1.10086 | 0.65207 | 2.47095 |
| | Submodel | Yes | 1.14731 | 0.68052 | 2.59951 |
| MSH2 | Full model | No | 1.19589 | 0.66774 | 2.57277 |
| | Full model | Yes | 1.18167 | 0.65659 | 2.54537 |
| | Submodel | No | 0.88121 | 0.48975 | 1.87265 |
| | Submodel | Yes | 0.88526 | 0.49393 | 1.88108 |
| MSH6 | Full model | No | 1.40642 | 0.62832 | 4.17756 |
| | Full model | Yes | 1.37141 | 0.60714 | 4.10324 |
| | Submodel | No | 0.55822 | 0.22502 | 1.70181 |
| | Submodel | Yes | 0.55872 | 0.22497 | 1.70180 |
| MMRpro genes | Full model | No | 1.09630 | 0.74284 | 1.72130 |
| | Full model | Yes | 1.10456 | 0.74708 | 1.72237 |
| | Submodel | No | 0.75711 | 0.51725 | 1.16758 |
| | Submodel | Yes | 0.76967 | 0.52367 | 1.17671 |
| PALB2 | Full model | No | 1.13199 | 0.55771 | 3.30646 |
| | Full model | Yes | 0.94977 | 0.45830 | 2.77960 |
| PMS2 | Full model | No | 0.76614 | 0.39242 | 1.68924 |
| | Full model | Yes | 0.75040 | 0.38006 | 1.64161 |
| Any BM | Full model | No | 0.75058 | 0.60447 | 0.92070 |
| | Full model | Yes | 1.10788 | 0.90988 | 1.33835 |
| | Submodel | No | 0.70376 | 0.57024 | 0.85805 |
| | Submodel | Yes | 1.06003 | 0.86313 | 1.28319 |
| Any | Full model | No | 0.75438 | 0.64312 | 0.88920 |
| | Full model | Yes | 0.97210 | 0.83210 | 1.13513 |

Table S7: (continued from previous page)

(c) Mean squared error (MSE).

| Gene | Model | Risk Modifiers | Estimate | Bootstrap 2.5% | Bootstrap 97.5% |
|---|---|---|---|---|---|
| ATM | Full model | No | 0.01204 | 0.00623 | 0.01802 |
| | Full model | Yes | 0.01199 | 0.00617 | 0.01791 |
| BRCA1 | Full model | No | 0.02895 | 0.02182 | 0.03730 |
| | Full model | Yes | 0.03740 | 0.02960 | 0.04584 |
| | Submodel | No | 0.02939 | 0.02221 | 0.03765 |
| | Submodel | Yes | 0.03765 | 0.02967 | 0.04627 |
| BRCA2 | Full model | No | 0.03055 | 0.02243 | 0.03947 |
| | Full model | Yes | 0.03019 | 0.02195 | 0.03888 |
| | Submodel | No | 0.03065 | 0.02241 | 0.03943 |
| | Submodel | Yes | 0.03025 | 0.02198 | 0.03887 |
| BRCAPRO genes | Full model | No | 0.05265 | 0.04278 | 0.06277 |
| | Full model | Yes | 0.05777 | 0.04845 | 0.06838 |
| | Submodel | No | 0.05313 | 0.04322 | 0.06341 |
| | Submodel | Yes | 0.05812 | 0.04869 | 0.06902 |
| CDKN2A | Full model | No | 0.00447 | 0.00139 | 0.00784 |
| | Full model | Yes | 0.00445 | 0.00138 | 0.00780 |
| | Submodel | No | 0.00188 | 0.00033 | 0.00392 |
| | Submodel | Yes | 0.00188 | 0.00033 | 0.00392 |
| CHEK2 | Full model | No | 0.01391 | 0.00833 | 0.02028 |
| | Full model | Yes | 0.01388 | 0.00832 | 0.02022 |
| EPCAM | Full model | No | 0.00305 | 0.00068 | 0.00597 |
| | Full model | Yes | 0.00305 | 0.00068 | 0.00597 |
| MLH1 | Full model | No | 0.00972 | 0.00530 | 0.01443 |
| | Full model | Yes | 0.00939 | 0.00499 | 0.01398 |
| | Submodel | No | 0.00653 | 0.00285 | 0.01037 |
| | Submodel | Yes | 0.00635 | 0.00270 | 0.01009 |
| MSH2 | Full model | No | 0.01071 | 0.00598 | 0.01610 |
| | Full model | Yes | 0.01064 | 0.00590 | 0.01602 |
| | Submodel | No | 0.00924 | 0.00484 | 0.01411 |
| | Submodel | Yes | 0.00918 | 0.00482 | 0.01404 |
| MSH6 | Full model | No | 0.00917 | 0.00451 | 0.01427 |
| | Full model | Yes | 0.00915 | 0.00450 | 0.01426 |
| | Submodel | No | 0.00624 | 0.00244 | 0.01059 |
| | Submodel | Yes | 0.00624 | 0.00244 | 0.01059 |
| MMRpro genes | Full model | No | 0.02401 | 0.01684 | 0.03133 |
| | Full model | Yes | 0.02368 | 0.01659 | 0.03095 |
| | Submodel | No | 0.02005 | 0.01331 | 0.02663 |
| | Submodel | Yes | 0.01987 | 0.01316 | 0.02649 |
| PALB2 | Full model | No | 0.00835 | 0.00375 | 0.01338 |
| | Full model | Yes | 0.00832 | 0.00377 | 0.01343 |
| PMS2 | Full model | No | 0.01072 | 0.00613 | 0.01665 |
| | Full model | Yes | 0.01071 | 0.00611 | 0.01664 |
| Any BM | Full model | No | 0.07242 | 0.06163 | 0.08420 |
| | Full model | Yes | 0.07738 | 0.06617 | 0.08885 |
| | Submodel | No | 0.07241 | 0.06103 | 0.08421 |
| | Submodel | Yes | 0.07754 | 0.06609 | 0.08982 |
| Any | Full model | No | 0.09817 | 0.08464 | 0.11032 |
| | Full model | Yes | 0.10253 | 0.08998 | 0.11518 |

# S7 Bootstraps where PanelPRO improves

In addition to looking directly at diagnostic metrics and their confidence intervals, another approach for evaluating model performance is by considering the fraction of bootstrap replicates where the full PanelPRO model improves in area under the curve (AUC), calibration (expected divided by observed number of events), and mean squared error (MSE) over the submodels in the BayesMendel package (BRCAPRO, MMRpro, and Melapro). This is the percentage of the 1000 bootstraps where PanelPRO's AUC and calibration are closer to 1 and where PanelPRO's MSE is closer to 0.

Tables S8 and S9 summarize the proportion of bootstraps where PanelPRO improves for the families simulated and evaluated under PanelPRO-5BC and PanelPRO-11, respectively. Tables S10 and S11 summarize these values for the HCP cohort families evaluated under PanelPRO-5BC and PanelPRO-11. Boxplots depicting the distributions of the percent improvement of PanelPRO compared to the submodel(s) in each bootstrap sample (no risk modifiers) are shown in Figures S6 and S7. A positive percent corresponds to a bootstrap sample where PanelPRO improves over the submodel, and vice-versa for negative percents.

In the HCP data, the results for PanelPRO-5BC and PanelPRO-11 appear to be mixed, with the bootstraps being frequently split or even in favor of the submodels. Looking at Figure S7, the differences between PanelPRO-5BC and BRCAPRO are typically quite small, with most percent changes less than 2%. The results comparing PanelPRO-11 and the BayesMendel submodels diverge noticeably more. The lack of consistent improvement is likely due to the limited size and ascertainment process for the HCP data. The cohort is high-risk and contains a high proportion of individuals with breast and ovarian cancer relative to other disease types. Therefore, many of the additional associations incorporated into PanelPRO-11 may not be easily detectable in this validation data set, despite being present in the general population. By inspecting some individual cases, we also observe that PanelPRO-11 often overpredicts the carrier probabilities for noncarriers with a strong family history of cancer, which could be attributable to genes not included in the model, polygenic risk, etc. As a result of these limitations in both the ascertainment process and the model, discrimination, calibration, and precision can be difficult.

The bootstraps for the PanelPRO-5BC simulated families tend to have better discrimination for PanelPRO-5BC but are less consistent in terms of calibration and precision. However, Figure S6 suggests that the differences are quite small and not especially significant. PanelPRO-11 improves upon nearly all of the bootstrap samples for the simulated families in terms of AUC and MSE, but has mixed results for calibration. The percent differences for calibration plotted in Figure S6 are still within 2% for most bootstraps.

Figure S8 plots the proportion of bootstraps where PanelPRO-11 improves in calibration over the submodels (no risk modifiers) in the simulated data as the number of simulated families increases from 1 million to 2 million. There is not really a consistent pattern across genes; the fraction of bootstraps where PanelPRO's calibration is better increases with the number of families for some genes, but not for others. The proportion of bootstraps where PanelPRO improves is likely not heavily dependent on the number of simulated families or counselees who are carriers, once a certain threshold in the number of families has been reached.

Figure S9 plots calibration against the number of carriers in the bootstrap sample, based on 1000 bootstraps of 2 million families simulated under PanelPRO-11 (no risk modifiers). The PanelPRO-11 calibrations are plotted as blue points and the BayesMendel calibrations are orange. Vertical lines connect calibrations of the same bootstrap sample, and are colored according to which model achieves a calibration closer to 1. For BRCA1 and BRCA2, PanelPRO yields a higher calibration compared to the submodel for any given bootstrap sample. This is also frequently the case for CDKN2A (76.8% of the bootstraps), MLH1 (86.2%), MSH2 (83.8%), and MSH6 (79.8%). Moreover, both models tend to underpredict when the the bootstraps sample has a lot of carriers, and to overpredict when the sample has few carriers. The relative performance of PanelPRO's calibration compared to that of the submodels appears to be largely dependent on to what extent both models are well-calibrated. In cases where the mean calibration across bootstraps is close to 1, the percent of bootstraps where PanelPRO improves will be close to 50%.

| Gene | Risk Modifiers | AUC | E/O | MSE |
|---|---|---|---|---|
| BRCA1 | No | 0.691 | 0.257 | 0.026 |
| | Yes | 0.973 | 1 | 0.996 |
| BRCA2 | No | 0.803 | 0.9 | 0.272 |
| | Yes | 0.805 | 0.291 | 0.415 |
| BRCAPRO genes | No | 0.854 | 0.586 | 0.376 |
| | Yes | 0.949 | 0.999 | 0.985 |

Table S8: Proportion of the 1000 bootstrap samples of families simulated based on PanelPRO-5BC where PanelPRO-5BC improves in area under the curve (AUC), calibration (expected divided by observed number of events, and mean squared error (MSE) over BRCAPRO. “BRCAPRO genes” indicates any of the genes in BRCAPRO (BRCA1, BRCA2).

| Gene | Risk Modifiers | AUC | E/O | MSE |
|---|---|---|---|---|
| BRCA1 | No | 0.999 | 0.358 | 0.97 |
| | Yes | 0.988 | 1 | 0.966 |
| BRCA2 | No | 0.998 | 0.462 | 0.998 |
| | Yes | 0.998 | 0.043 | 0.998 |
| BRCAPRO genes | No | 1 | 0.281 | 1 |
| | Yes | 1 | 0.982 | 1 |
| CDKN2A | No | 1 | 0.547 | 0.998 |
| | Yes | 1 | 0.547 | 0.998 |
| MLH1 | No | 1 | 0.567 | 1 |
| | Yes | 1 | 0.499 | 1 |
| MSH2 | No | 1 | 0.436 | 1 |
| | Yes | 1 | 0.615 | 1 |
| MSH6 | No | 1 | 0.881 | 0.903 |
| | Yes | 1 | 0.931 | 0.986 |
| MMRpro genes | No | 1 | 0.441 | 1 |
| | Yes | 1 | 0.549 | 1 |
| Any BM | No | 1 | 0.146 | 1 |
| | Yes | 1 | 0.868 | 1 |

Table S9: Proportion of the 1000 bootstrap samples of families simulated based on PanelPRO-11 where PanelPRO-11 improves in area under the curve (AUC), calibration (expected divided by observed number of events, and mean squared error (MSE) over BRCAPRO, MMRpro, and Melapro. “BRCAPRO genes”, “MMRpro genes”, and “Any BM” indicate any of the genes in BRCAPRO (BRCA1, BRCA2), MMRpro (MLH1, MSH2, MSH6), and any model in the BayesMendel package (BRCA1, BRCA2, MLH1, MSH2, MSH6, CDKN2A), respectively.

| Gene | Risk Modifiers | AUC | E/O | MSE |
|---|---|---|---|---|
| BRCA1 | No | 0.799 | 0.051 | 0.988 |
| | Yes | 0.814 | 0.937 | 0.929 |
| BRCA2 | No | 0.357 | 0.164 | 0.969 |
| | Yes | 0.588 | 0.065 | 0.983 |
| BRCAPRO genes | No | 0.669 | 0.006 | 0.987 |
| | Yes | 0.54 | 0.363 | 0.791 |

Table S10: Proportion of the 1000 bootstrap samples of the HCP cohort families where PanelPRO-5BC improves in area under the curve (AUC), calibration (expected divided by observed number of events, and mean squared error (MSE) over BRCAPRO. “BRCAPRO genes” indicates any of the genes in BRCAPRO (BRCA1, BRCA2).

| Gene | Risk Modifiers | AUC | E/O | MSE |
|---|---|---|---|---|
| BRCA1 | No | 0.653 | 0.026 | 0.987 |
| | Yes | 0.597 | 0.601 | 0.776 |
| BRCA2 | No | 0.32 | 0.096 | 0.622 |
| | Yes | 0.279 | 0.227 | 0.577 |
| BRCAPRO genes | No | 0.467 | 0.151 | 0.851 |
| | Yes | 0.215 | 0.286 | 0.755 |
| CDKN2A | No | 0 | 0.38 | 0.018 |
| | Yes | 0 | 0.382 | 0.018 |
| MLH1 | No | 0.155 | 0.156 | 0.005 |
| | Yes | 0.163 | 0.119 | 0.006 |
| MSH2 | No | 0.223 | 0.452 | 0.159 |
| | Yes | 0.261 | 0.463 | 0.16 |
| MSH6 | No | 0.016 | 0.498 | 0.002 |
| | Yes | 0.015 | 0.521 | 0.004 |
| MMRpro genes | No | 0 | 0.646 | 0.001 |
| | Yes | 0.002 | 0.633 | 0.002 |
| Any BM | No | 0.751 | 0.99 | 0.495 |
| | Yes | 0.565 | 0.193 | 0.556 |

Table S11: Proportion of the 1000 bootstrap samples of the HCP cohort families where PanelPRO-11 improves in area under the curve (AUC), calibration (expected divided by observed number of events, and mean squared error (MSE) over BRCAPRO, MMRpro, and Melapro. "BRCAPRO genes", "MMRpro genes", and "Any BM" indicate any of the genes in BRCAPRO (BRCA1, BRCA2), MMRpro (MLH1, MSH2, MSH6), and any model in the BayesMendel package (BRCA1, BRCA2, MLH1, MSH2, MSH6, CDKN2A), respectively.

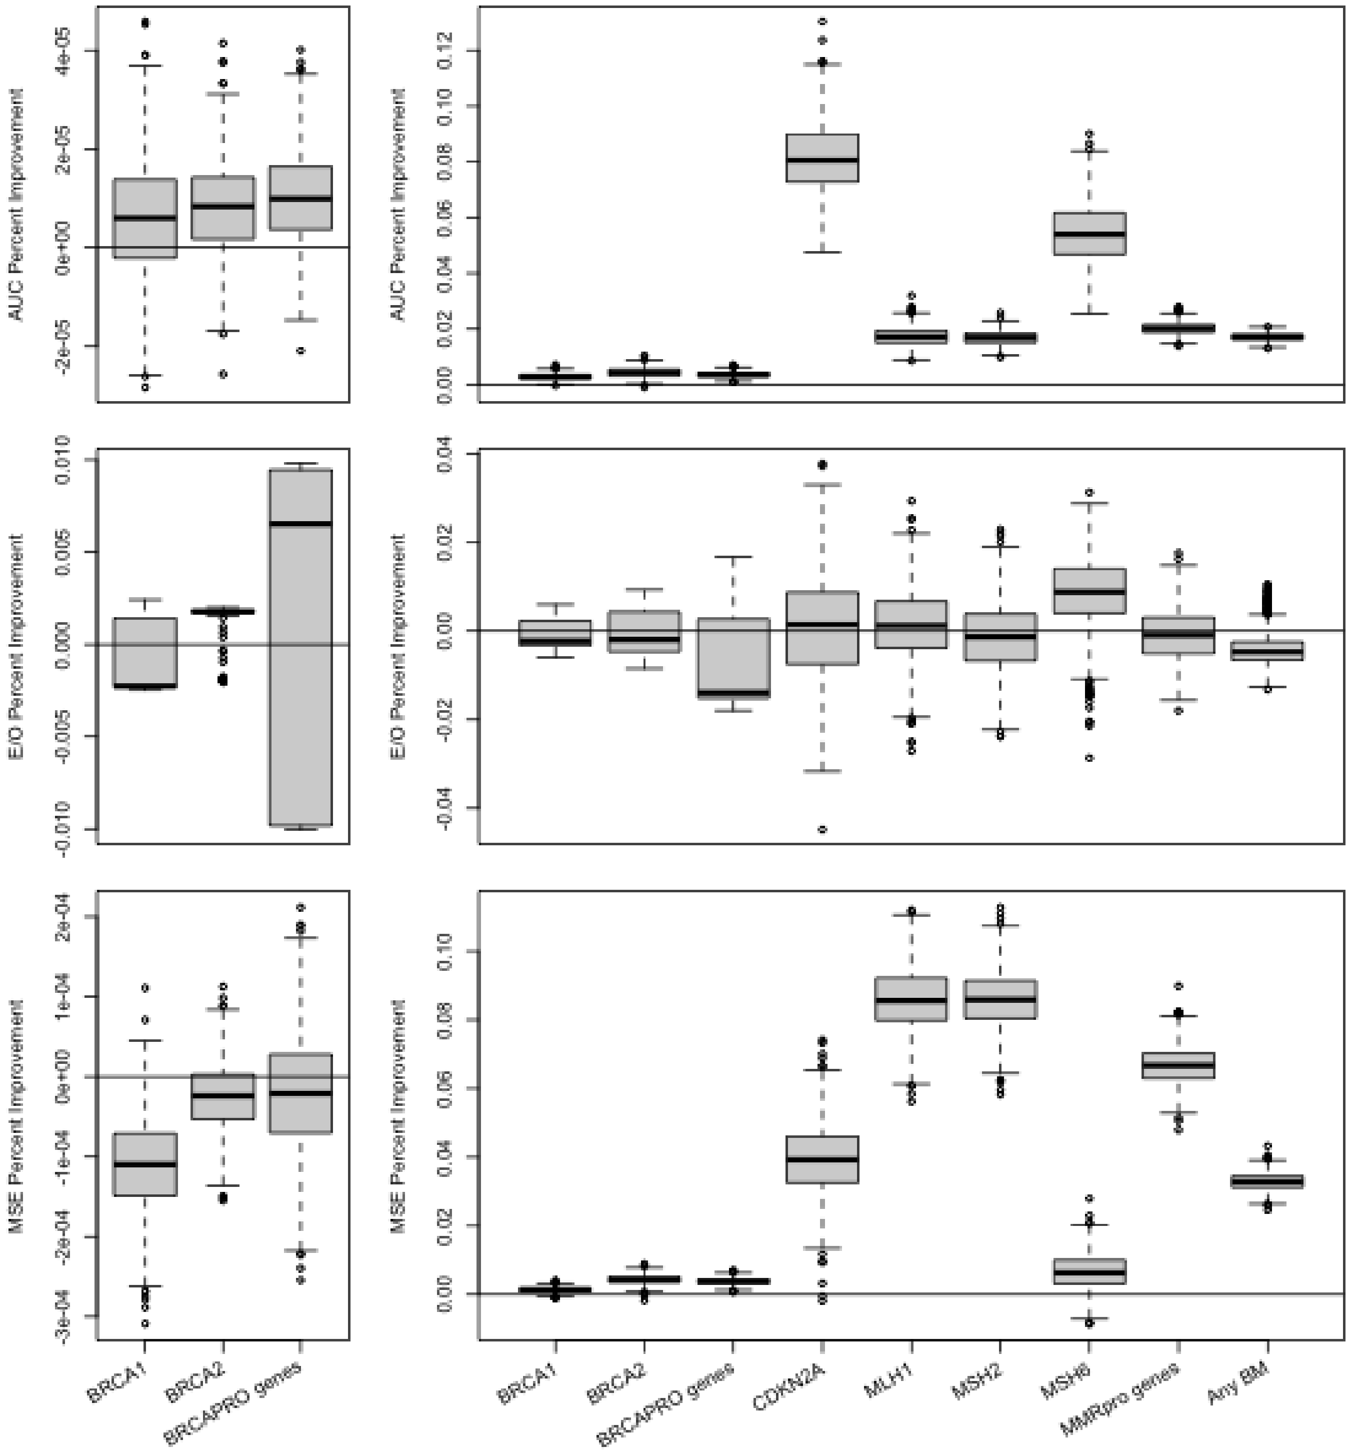


Figure S6: Distribution of the percent improvement in area under the curve (AUC), calibration (expected divided by observed number of events), and mean squared error (MSE) that PanelPRO makes over the models in the BayesMendel package (BRCAPRO, MMRpro, and Melapro). The distributions are over the 1000 bootstrap samples of families simulated and evaluated under PanelPRO-5BC (left) and PanelPRO-11 (right). A positive percent is considered an improvement of PanelPRO over the submodel; a negative percent is considered an improvement of the submodel over PanelPRO.

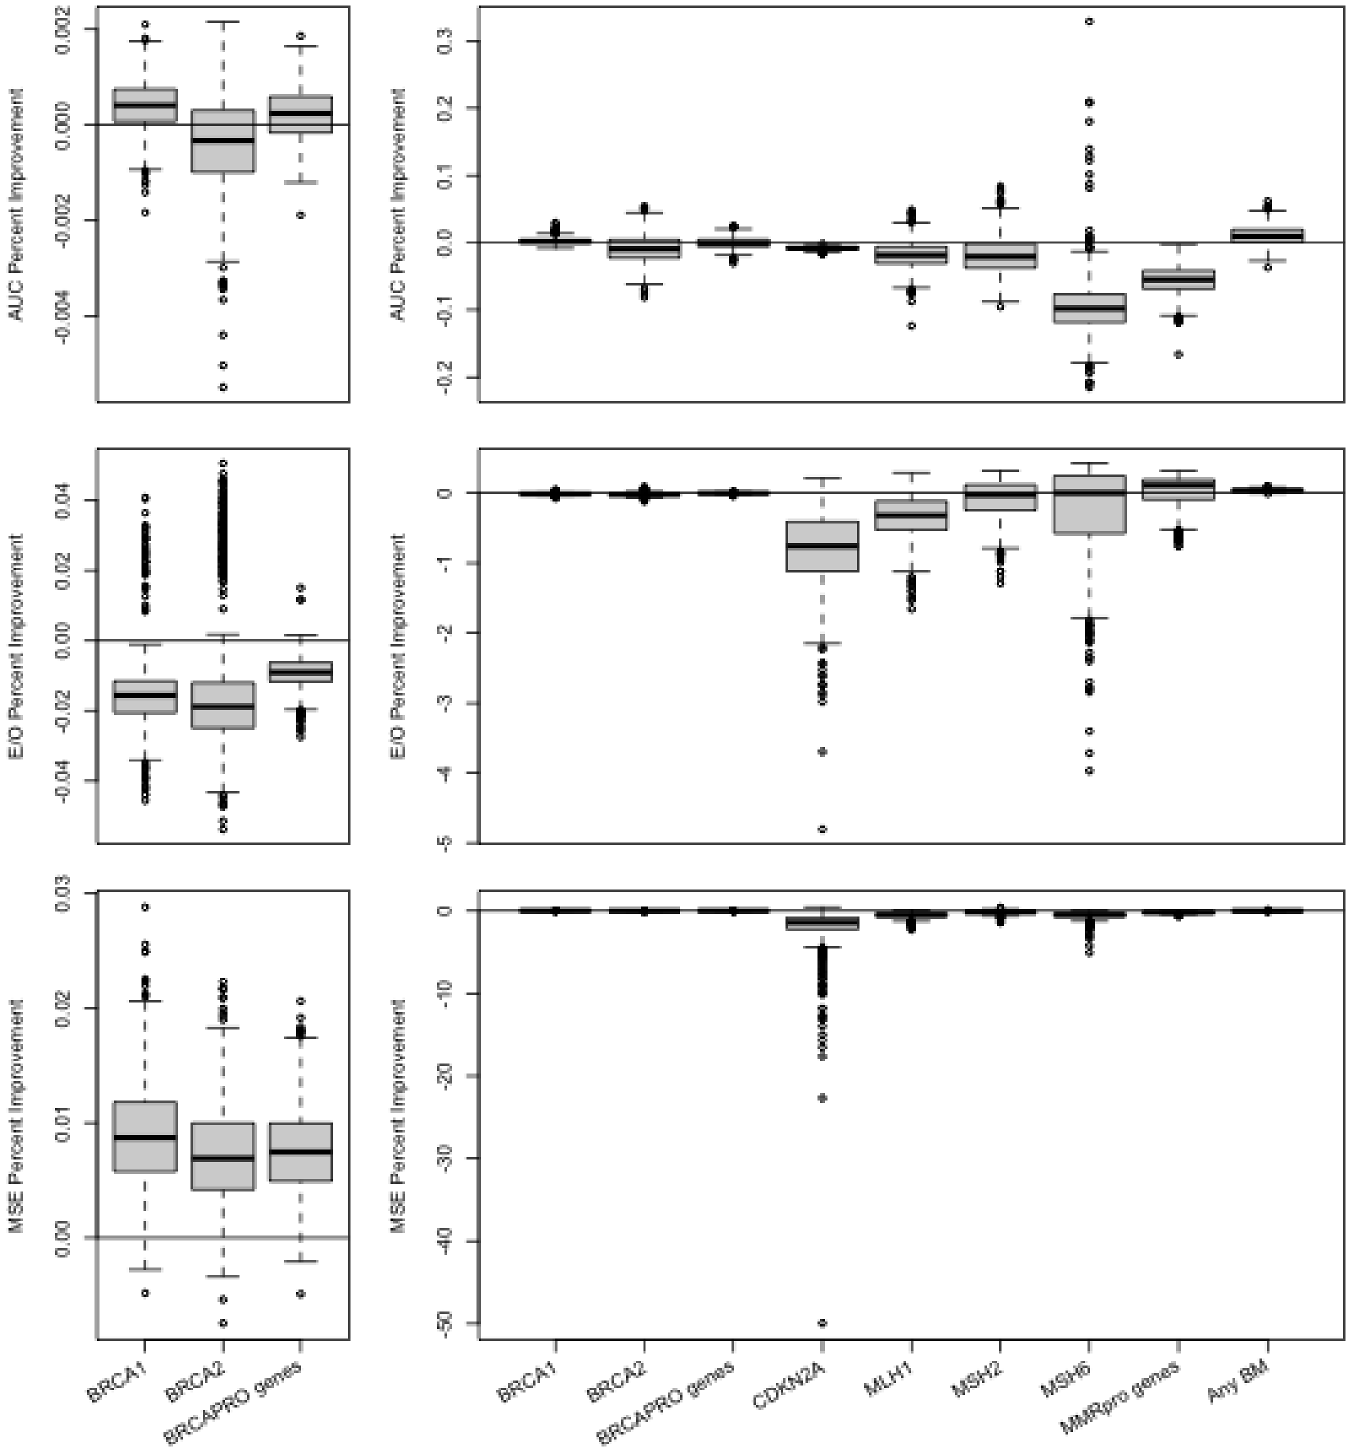


Figure S7: Distribution of the percent improvement in area under the curve (AUC), calibration (expected divided by observed number of events), and mean squared error (MSE) that PanelPRO makes over the models in the BayesMendel package (BRCAPRO, MMRpro, and Melapro). The distributions are over the 1000 bootstrap samples of the HCP cohort families evaluated under PanelPRO-5BC (left) and PanelPRO-11 (right). A positive percent is considered an improvement of PanelPRO over the submodel; a negative percent is considered an improvement of the submodel over PanelPRO.

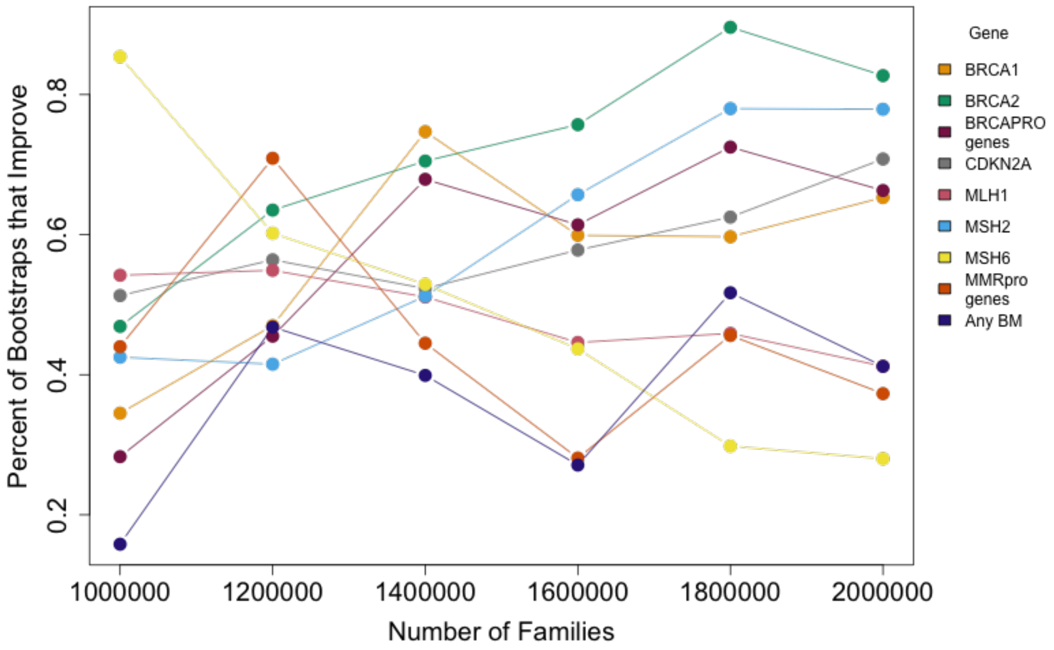


Figure S8: Proportion of 1000 bootstraps where PanelPRO-11 improves upon calibration (expected divided by observed number of events) compared to the models in the BayesMendel package (BRCAPRO, MMRpro, and Melapro) plotted against number of simulated families.

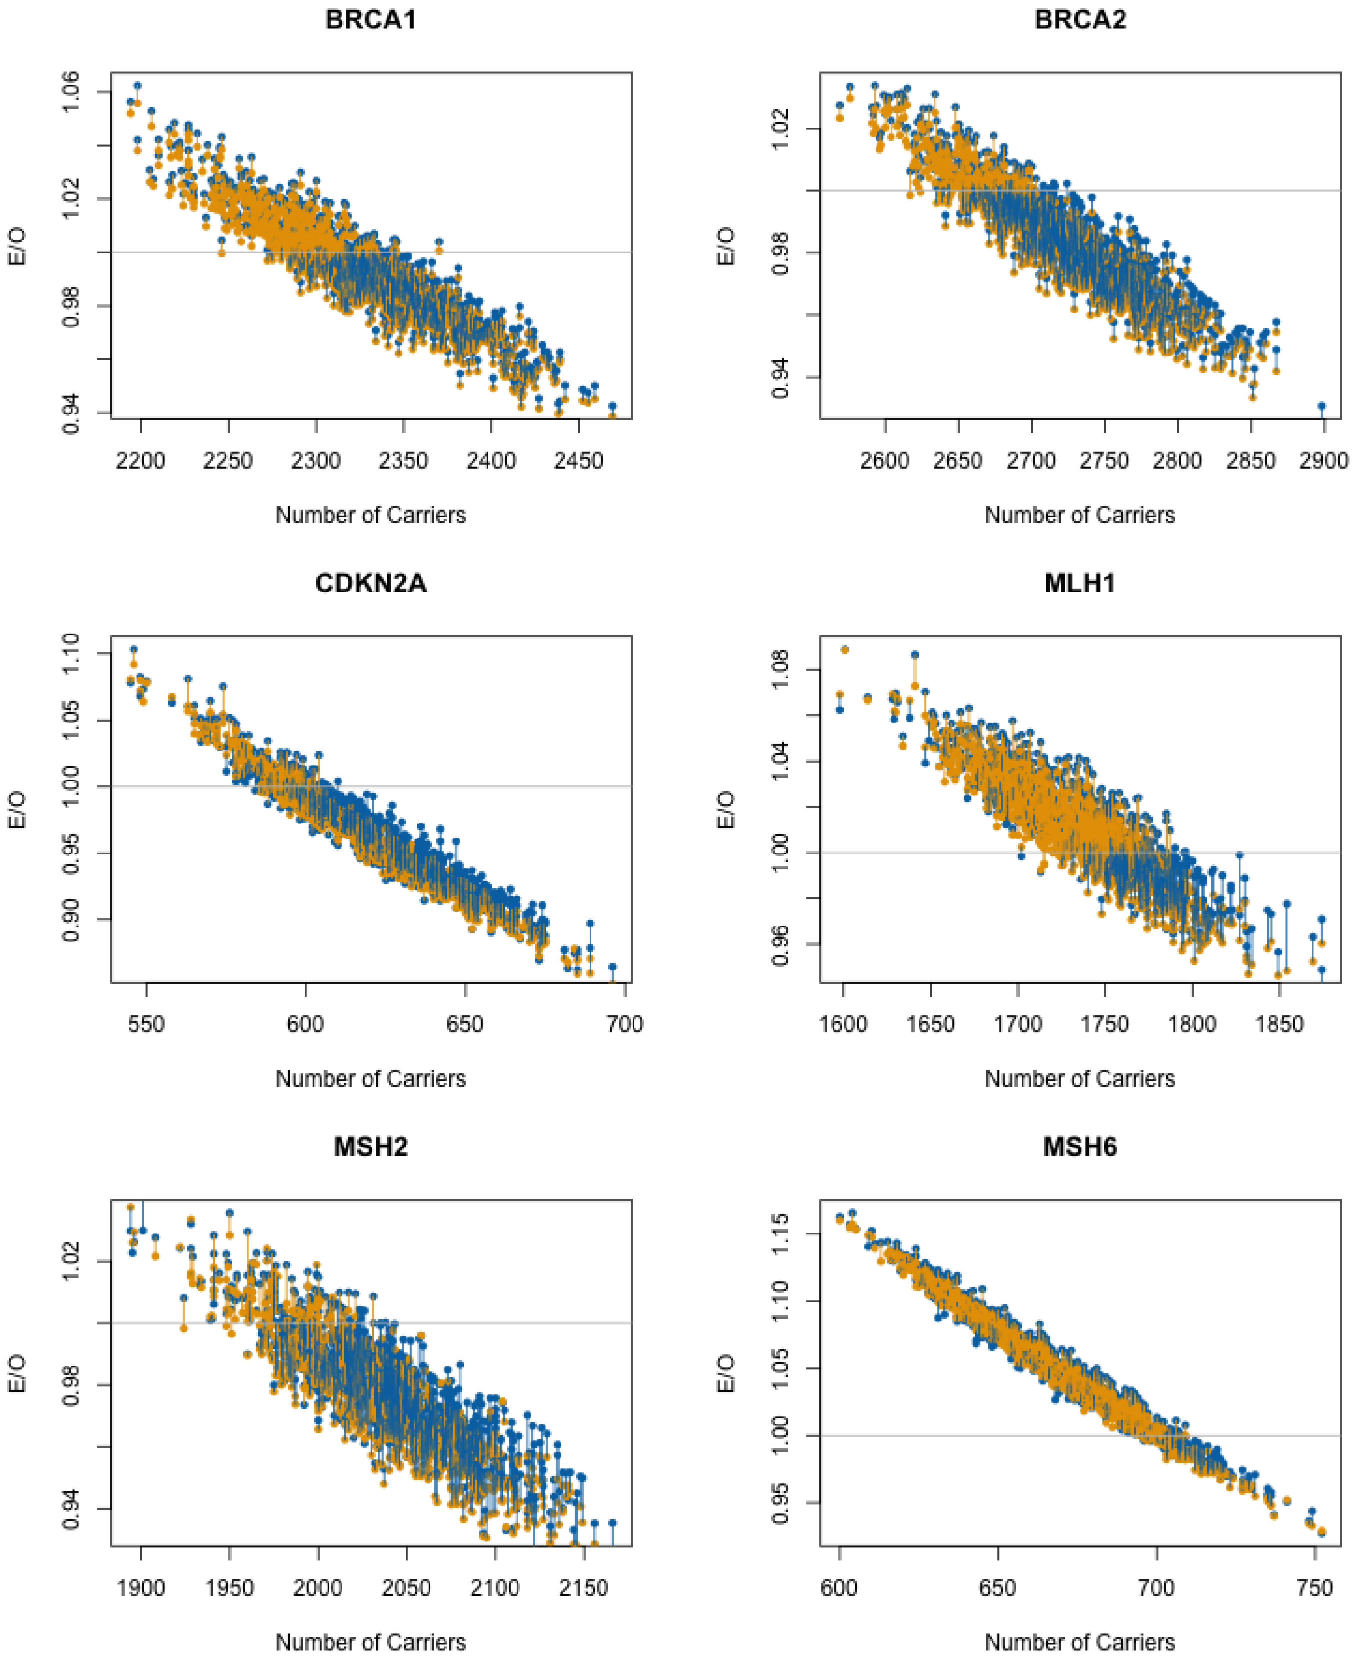


Figure S9: Plot of calibration (expected divided by observed number of events) against the number of carriers in the bootstrap sample, based on 1000 bootstraps of 2 million families simulated under PanelPRO-11. The PanelPRO-11 calibrations are plotted as blue points and the calibrations from the models in the BayesMendel package (BRCAPRO, MMRpro, and Melapro) are orange. Vertical lines connect calibrations of the same bootstrap sample, and are colored according to which model achieves a calibration closer to 1.

## S8 PanelPRO-5BC Sensitivity to Family Size

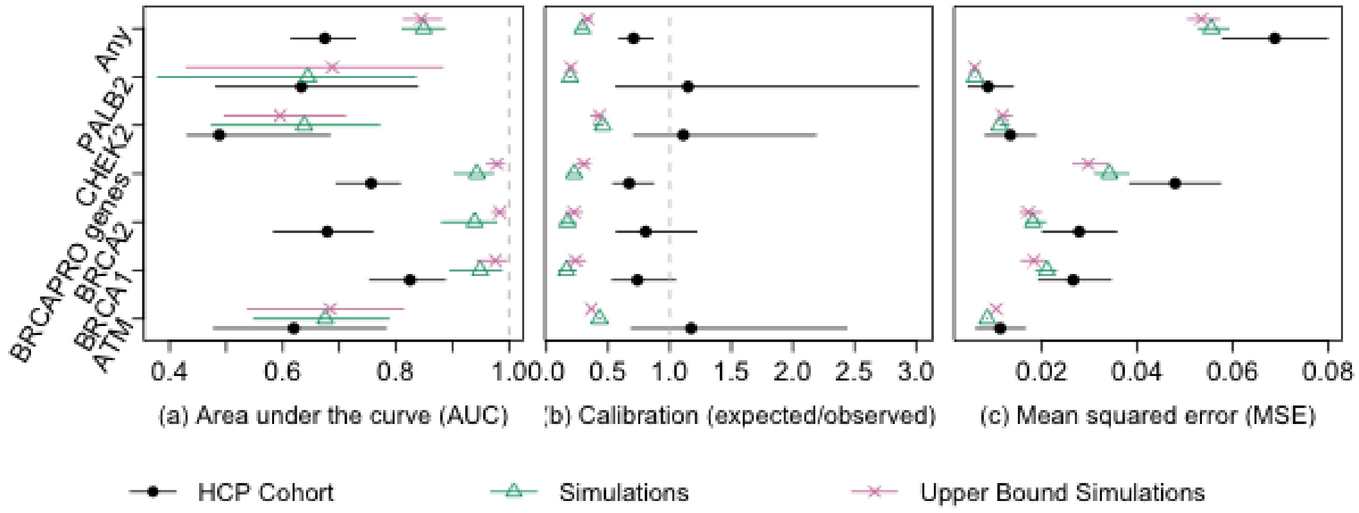


Figure S10: AUC, calibration, and MSE for PanelPRO-5BC evaluated on the HCP cohort (black closed circles), simulated families with structures sampled from the HCP cohort (green open triangles), and large simulated families (purple crosses). "BRCAPRO genes" indicates any of the genes in BRCAPRO (BRCA1, BRCA2), and "Any" indicates any of the five genes in PanelPRO-5BC. 95% bootstrap percentile confidence intervals are also shown.

Table S12: AUC, calibration, and MSE for PanelPRO-5BC evaluated on the HCP cohort, simulated families with structures sampled from the HCP cohort, and large simulated families. "BRCAPRO genes" indicates any of the genes in BRCAPRO (BRCA1, BRCA2), and "Any" indicates any of the five genes in PanelPRO-5BC. 95% bootstrap percentile confidence intervals are also reported.

(a) Area under the curve (AUC).

| Gene | Data | Estimate | Bootstrap 2.5% | Bootstrap 97.5% |
|---|---|---|---|---|
| ATM | HCP Cohort | 0.61944 | 0.47854 | 0.78247 |
| | Simulations | 0.67521 | 0.54890 | 0.78747 |
| | Upper Bound Simulations | 0.68398 | 0.53740 | 0.81354 |
| BRCA1 | HCP Cohort | 0.82502 | 0.75408 | 0.88664 |
| | Simulations | 0.94881 | 0.89614 | 0.98673 |
| | Upper Bound Simulations | 0.97559 | 0.94373 | 0.99530 |
| BRCA2 | HCP Cohort | 0.67855 | 0.58382 | 0.75894 |
| | Simulations | 0.93910 | 0.88090 | 0.97719 |
| | Upper Bound Simulations | 0.98330 | 0.97014 | 0.99343 |
| BRCAPRO genes | HCP Cohort | 0.75616 | 0.69464 | 0.80701 |
| | Simulations | 0.94309 | 0.90373 | 0.97221 |
| | Upper Bound Simulations | 0.97871 | 0.96020 | 0.99159 |
| CHEK2 | HCP Cohort | 0.48791 | 0.43141 | 0.68304 |
| | Simulations | 0.63799 | 0.47441 | 0.77093 |
| | Upper Bound Simulations | 0.59535 | 0.49734 | 0.71037 |
| PALB2 | HCP Cohort | 0.63279 | 0.48168 | 0.83771 |
| | Simulations | 0.64427 | 0.37924 | 0.83462 |
| | Upper Bound Simulations | 0.68758 | 0.43024 | 0.88207 |
| Any | HCP Cohort | 0.67436 | 0.61491 | 0.72804 |
| | Simulations | 0.84923 | 0.81137 | 0.88630 |
| | Upper Bound Simulations | 0.84469 | 0.81324 | 0.87977 |

Table S12: (continued from previous page)

(b) Calibration (expected divided by observed number of events).

| Gene | Data | Estimate | Bootstrap 2.5% | Bootstrap 97.5% |
|---|---|---|---|---|
| ATM | HCP Cohort | 1.17429 | 0.68925 | 2.43607 |
| | Simulations | 0.43041 | 0.42235 | 0.43909 |
| | Upper Bound Simulations | 0.36377 | 0.35288 | 0.37609 |
| BRCA1 | HCP Cohort | 0.73783 | 0.53406 | 1.04564 |
| | Simulations | 0.16317 | 0.10327 | 0.23982 |
| | Upper Bound Simulations | 0.23727 | 0.17248 | 0.31572 |
| BRCA2 | HCP Cohort | 0.80527 | 0.56862 | 1.21781 |
| | Simulations | 0.17109 | 0.11444 | 0.23502 |
| | Upper Bound Simulations | 0.22436 | 0.15718 | 0.28981 |
| BRCAPRO genes | HCP Cohort | 0.67139 | 0.53990 | 0.86996 |
| | Simulations | 0.22549 | 0.17036 | 0.27876 |
| | Upper Bound Simulations | 0.30397 | 0.24820 | 0.35627 |
| CHEK2 | HCP Cohort | 1.11064 | 0.70807 | 2.18568 |
| | Simulations | 0.45717 | 0.38680 | 0.46178 |
| | Upper Bound Simulations | 0.42958 | 0.36526 | 0.43479 |
| PALB2 | HCP Cohort | 1.14825 | 0.56474 | 3.01631 |
| | Simulations | 0.19242 | 0.18359 | 0.20289 |
| | Upper Bound Simulations | 0.19831 | 0.18643 | 0.21157 |
| Any | HCP Cohort | 0.70763 | 0.58871 | 0.86623 |
| | Simulations | 0.29236 | 0.25488 | 0.32666 |
| | Upper Bound Simulations | 0.33396 | 0.29783 | 0.36824 |

(c) Mean squared error (MSE).

| Gene | Data | Estimate | Bootstrap 2.5% | Bootstrap 97.5% |
|---|---|---|---|---|
| ATM | HCP Cohort | 0.01126 | 0.00617 | 0.01642 |
| | Simulations | 0.00855 | 0.00854 | 0.00856 |
| | Upper Bound Simulations | 0.01039 | 0.01034 | 0.01043 |
| BRCA1 | HCP Cohort | 0.02653 | 0.01930 | 0.03443 |
| | Simulations | 0.02102 | 0.01876 | 0.02302 |
| | Upper Bound Simulations | 0.01830 | 0.01572 | 0.02039 |
| BRCA2 | HCP Cohort | 0.02779 | 0.02014 | 0.03561 |
| | Simulations | 0.01807 | 0.01659 | 0.02072 |
| | Upper Bound Simulations | 0.01716 | 0.01550 | 0.01982 |
| BRCAPRO genes | HCP Cohort | 0.04787 | 0.03839 | 0.05735 |
| | Simulations | 0.03412 | 0.03110 | 0.03809 |
| | Upper Bound Simulations | 0.02972 | 0.02654 | 0.03382 |
| CHEK2 | HCP Cohort | 0.01337 | 0.00810 | 0.01871 |
| | Simulations | 0.01112 | 0.01110 | 0.01306 |
| | Upper Bound Simulations | 0.01169 | 0.01169 | 0.01362 |
| PALB2 | HCP Cohort | 0.00868 | 0.00459 | 0.01390 |
| | Simulations | 0.00595 | 0.00594 | 0.00596 |
| | Upper Bound Simulations | 0.00590 | 0.00588 | 0.00592 |
| Any | HCP Cohort | 0.06876 | 0.05784 | 0.07980 |
| | Simulations | 0.05547 | 0.05283 | 0.05905 |
| | Upper Bound Simulations | 0.05338 | 0.05054 | 0.05706 |

## S9 PanelPRO-11 Sensitivity to Family Size

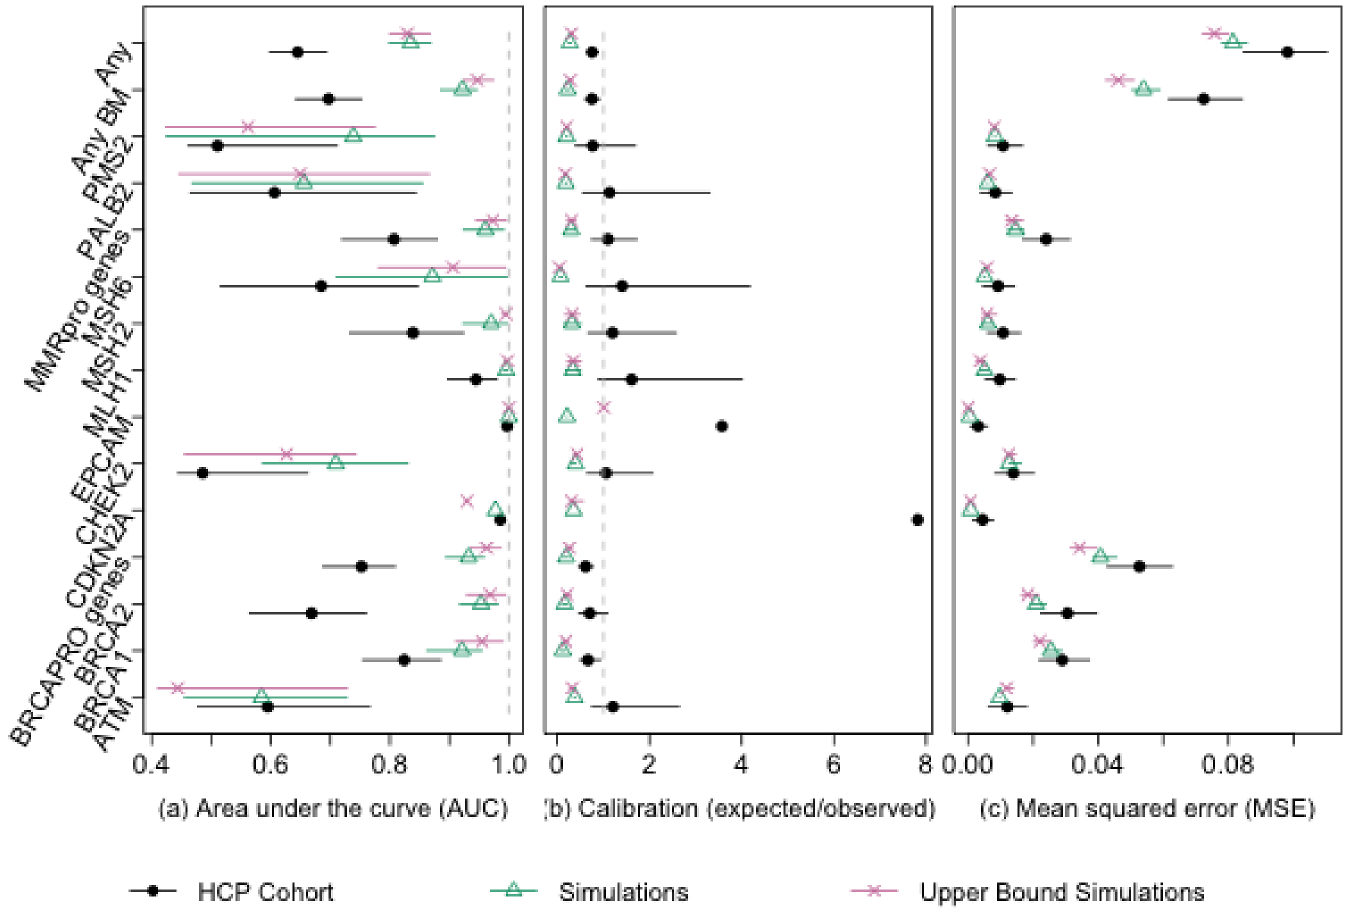


Figure S11: AUC, calibration, and MSE for PanelPRO-11 evaluated on the HCP cohort (black closed circles), simulated families with structures sampled from the HCP cohort (green open triangles), and large simulated families (purple crosses). "BRCAPRO genes", "MMRpro genes", and "Any BM" indicate any of the genes in BRCAPRO (BRCA1, BRCA2), MMRpro (MLH1, MSH2, MSH6), and any model in the BayesMendel package (BRCA1, BRCA2, MLH1, MSH2, MSH6, CDKN2A), respectively. "Any" indicates any of the eleven genes in PanelPRO-11. 95% bootstrap percentile confidence intervals are also shown.

Table S13: AUC, calibration, and MSE for PanelPRO-11 evaluated on the HCP cohort, simulated families with structures sampled from the HCP cohort, and large simulated families. "BRCAPRO genes", "MMRpro genes", and "Any BM" indicate any of the genes in BRCAPRO (BRCA1, BRCA2), MMRpro (MLH1, MSH2, MSH6), and any model in the BayesMendel package (BRCA1, BRCA2, MLH1, MSH2, MSH6, CDKN2A), respectively. "Any" indicates any of the eleven genes in PanelPRO-11. 95% bootstrap percentile confidence intervals are also reported.

(a) Area under the curve (AUC).

| Gene | Data | Estimate | Bootstrap 2.5% | Bootstrap 97.5% |
|---|---|---|---|---|
| ATM | HCP Cohort | 0.59478 | 0.47680 | 0.76613 |
| | Simulations | 0.58446 | 0.45493 | 0.72751 |
| | Upper Bound Simulations | 0.44344 | 0.41002 | 0.72798 |
| BRCA1 | HCP Cohort | 0.82414 | 0.75479 | 0.88541 |
| | Simulations | 0.92116 | 0.86231 | 0.95474 |
| | Upper Bound Simulations | 0.95487 | 0.91058 | 0.99022 |
| BRCA2 | HCP Cohort | 0.66842 | 0.56442 | 0.76003 |
| | Simulations | 0.95317 | 0.91765 | 0.98135 |
| | Upper Bound Simulations | 0.96834 | 0.92903 | 0.99414 |
| BRCAPRO genes | HCP Cohort | 0.75229 | 0.68726 | 0.80875 |
| | Simulations | 0.93221 | 0.89387 | 0.95850 |
| | Upper Bound Simulations | 0.96235 | 0.93538 | 0.98635 |
| CDKN2A | HCP Cohort | 0.98558 | 0.97939 | 0.99177 |
| | Simulations | 0.97720 | 0.97720 | 0.97720 |
| | Upper Bound Simulations | 0.92969 | 0.92605 | 0.92818 |
| CHEK2 | HCP Cohort | 0.48543 | 0.44348 | 0.66200 |
| | Simulations | 0.70919 | 0.58619 | 0.83033 |
| | Upper Bound Simulations | 0.62638 | 0.45516 | 0.74266 |
| EPCAM | HCP Cohort | 0.99697 | 0.99394 | 0.99957 |
| | Simulations | 1.00000 | 1.00000 | 1.00000 |
| | Upper Bound Simulations | 1.00000 | 1.00000 | 1.00000 |
| MLH1 | HCP Cohort | 0.94470 | 0.89722 | 0.97960 |
| | Simulations | 0.99536 | 0.99115 | 0.99856 |
| | Upper Bound Simulations | 0.99767 | 0.99344 | 1.00000 |
| MSH2 | HCP Cohort | 0.83881 | 0.73263 | 0.92378 |
| | Simulations | 0.97023 | 0.92260 | 0.99710 |
| | Upper Bound Simulations | 0.99514 | 0.98815 | 0.99820 |
| MSH6 | HCP Cohort | 0.68448 | 0.51526 | 0.84725 |
| | Simulations | 0.87158 | 0.71003 | 0.99707 |
| | Upper Bound Simulations | 0.90604 | 0.78091 | 0.99422 |
| MMRpro genes | HCP Cohort | 0.80692 | 0.71909 | 0.87900 |
| | Simulations | 0.96051 | 0.92328 | 0.99163 |
| | Upper Bound Simulations | 0.97282 | 0.94476 | 0.99567 |
| PALB2 | HCP Cohort | 0.60613 | 0.46485 | 0.84361 |
| | Simulations | 0.65549 | 0.46826 | 0.85507 |
| | Upper Bound Simulations | 0.64880 | 0.44583 | 0.86614 |
| PMS2 | HCP Cohort | 0.51035 | 0.46136 | 0.71145 |
| | Simulations | 0.73867 | 0.42433 | 0.87481 |
| | Upper Bound Simulations | 0.56157 | 0.42370 | 0.77471 |
| Any BM | HCP Cohort | 0.69701 | 0.64183 | 0.75275 |
| | Simulations | 0.92200 | 0.88555 | 0.94639 |
| | Upper Bound Simulations | 0.94724 | 0.92418 | 0.97426 |
| Any | HCP Cohort | 0.64489 | 0.59798 | 0.69337 |
| | Simulations | 0.83476 | 0.79897 | 0.86861 |
| | Upper Bound Simulations | 0.82942 | 0.80021 | 0.86721 |

Table S13: (continued from previous page)

(b) Calibration (expected divided by observed number of events).

| Gene | Data | Estimate | Bootstrap 2.5% | Bootstrap 97.5% |
|---|---|---|---|---|
| ATM | HCP Cohort | 1.20604 | 0.74641 | 2.64397 |
| | Simulations | 0.37783 | 0.36230 | 0.39366 |
| | Upper Bound Simulations | 0.32357 | 0.26793 | 0.33578 |
| BRCA1 | HCP Cohort | 0.66618 | 0.49216 | 0.93316 |
| | Simulations | 0.11841 | 0.07454 | 0.16518 |
| | Upper Bound Simulations | 0.18395 | 0.12396 | 0.24705 |
| BRCA2 | HCP Cohort | 0.70521 | 0.47346 | 1.08308 |
| | Simulations | 0.15789 | 0.10402 | 0.21379 |
| | Upper Bound Simulations | 0.20961 | 0.16068 | 0.29375 |
| BRCAPRO genes | HCP Cohort | 0.61319 | 0.47020 | 0.78285 |
| | Simulations | 0.19216 | 0.14312 | 0.23385 |
| | Upper Bound Simulations | 0.26210 | 0.21766 | 0.31982 |
| CDKN2A | HCP Cohort | 7.81779 | 1.66689 | 7.81779 |
| | Simulations | 0.35436 | 0.35436 | 0.35436 |
| | Upper Bound Simulations | 0.30823 | 0.30301 | 0.56186 |
| CHEK2 | HCP Cohort | 1.05752 | 0.64159 | 2.07377 |
| | Simulations | 0.39495 | 0.30526 | 0.40051 |
| | Upper Bound Simulations | 0.43401 | 0.35780 | 0.45120 |
| EPCAM | HCP Cohort | 3.57143 | 0.42806 | 0.42806 |
| | Simulations | 0.21147 | 0.21049 | 0.21173 |
| | Upper Bound Simulations | 1.00676 | 1.00676 | 1.00676 |
| MLH1 | HCP Cohort | 1.61178 | 0.89169 | 4.00383 |
| | Simulations | 0.33301 | 0.18636 | 0.50394 |
| | Upper Bound Simulations | 0.35028 | 0.21611 | 0.51146 |
| MSH2 | HCP Cohort | 1.19589 | 0.66774 | 2.57277 |
| | Simulations | 0.31591 | 0.14020 | 0.51452 |
| | Upper Bound Simulations | 0.32601 | 0.15871 | 0.48383 |
| MSH6 | HCP Cohort | 1.40642 | 0.62832 | 4.17756 |
| | Simulations | 0.06973 | 0.04854 | 0.10480 |
| | Upper Bound Simulations | 0.04435 | 0.03548 | 0.05447 |
| MMRpro genes | HCP Cohort | 1.09630 | 0.74284 | 1.72130 |
| | Simulations | 0.29900 | 0.19981 | 0.40556 |
| | Upper Bound Simulations | 0.31271 | 0.21058 | 0.39850 |
| PALB2 | HCP Cohort | 1.13199 | 0.55771 | 3.30646 |
| | Simulations | 0.18631 | 0.17242 | 0.20050 |
| | Upper Bound Simulations | 0.17118 | 0.16007 | 0.18257 |
| PMS2 | HCP Cohort | 0.76614 | 0.39242 | 1.68924 |
| | Simulations | 0.20322 | 0.19411 | 0.21231 |
| | Upper Bound Simulations | 0.20253 | 0.18931 | 0.21741 |
| Any BM | HCP Cohort | 0.75058 | 0.60447 | 0.92070 |
| | Simulations | 0.22477 | 0.17993 | 0.26796 |
| | Upper Bound Simulations | 0.28081 | 0.24189 | 0.33130 |
| Any | HCP Cohort | 0.75438 | 0.64312 | 0.88920 |
| | Simulations | 0.27153 | 0.23981 | 0.29928 |
| | Upper Bound Simulations | 0.31061 | 0.27982 | 0.34057 |

Table S13: (continued from previous page)

(c) Mean squared error (MSE).

| Gene | Data | Estimate | Bootstrap 2.5% | Bootstrap 97.5% |
| --- | --- | --- | --- | --- |
| ATM | HCP Cohort | 0.01204 | 0.00623 | 0.01802 |
| | Simulations | 0.00969 | 0.00958 | 0.00974 |
| | Upper Bound Simulations | 0.01172 | 0.01165 | 0.01391 |
| BRCA1 | HCP Cohort | 0.02895 | 0.02182 | 0.03730 |
| | Simulations | 0.02543 | 0.02375 | 0.02874 |
| | Upper Bound Simulations | 0.02207 | 0.02017 | 0.02539 |
| BRCA2 | HCP Cohort | 0.03055 | 0.02243 | 0.03947 |
| | Simulations | 0.02087 | 0.01937 | 0.02392 |
| | Upper Bound Simulations | 0.01835 | 0.01645 | 0.02173 |
| BRCAPRO genes | HCP Cohort | 0.05265 | 0.04278 | 0.06277 |
| | Simulations | 0.04067 | 0.03850 | 0.04561 |
| | Upper Bound Simulations | 0.03426 | 0.03150 | 0.03950 |
| CDKN2A | HCP Cohort | 0.00447 | 0.00139 | 0.00784 |
| | Simulations | 0.00076 | 0.00000 | 0.00002 |
| | Upper Bound Simulations | 0.00075 | 0.00000 | 0.00001 |
| CHEK2 | HCP Cohort | 0.01391 | 0.00833 | 0.02028 |
| | Simulations | 0.01257 | 0.01253 | 0.01622 |
| | Upper Bound Simulations | 0.01244 | 0.01238 | 0.01461 |
| EPCAM | HCP Cohort | 0.00305 | 0.00068 | 0.00597 |
| | Simulations | 0.00048 | 0.00000 | 0.00000 |
| | Upper Bound Simulations | 0.00000 | 0.00000 | 0.00000 |
| MLH1 | HCP Cohort | 0.00972 | 0.00530 | 0.01443 |
| | Simulations | 0.00503 | 0.00364 | 0.00635 |
| | Upper Bound Simulations | 0.00372 | 0.00248 | 0.00502 |
| MSH2 | HCP Cohort | 0.01071 | 0.00598 | 0.01610 |
| | Simulations | 0.00609 | 0.00427 | 0.00764 |
| | Upper Bound Simulations | 0.00580 | 0.00448 | 0.00877 |
| MSH6 | HCP Cohort | 0.00917 | 0.00451 | 0.01427 |
| | Simulations | 0.00508 | 0.00475 | 0.00526 |
| | Upper Bound Simulations | 0.00587 | 0.00579 | 0.00592 |
| MMRpro genes | HCP Cohort | 0.02401 | 0.01684 | 0.03133 |
| | Simulations | 0.01458 | 0.01222 | 0.01698 |
| | Upper Bound Simulations | 0.01344 | 0.01174 | 0.01677 |
| PALB2 | HCP Cohort | 0.00835 | 0.00375 | 0.01338 |
| | Simulations | 0.00602 | 0.00600 | 0.00603 |
| | Upper Bound Simulations | 0.00666 | 0.00664 | 0.00667 |
| PMS2 | HCP Cohort | 0.01072 | 0.00613 | 0.01665 |
| | Simulations | 0.00825 | 0.00822 | 0.00826 |
| | Upper Bound Simulations | 0.00802 | 0.00783 | 0.00813 |
| Any BM | HCP Cohort | 0.07242 | 0.06163 | 0.08420 |
| | Simulations | 0.05394 | 0.05051 | 0.05895 |
| | Upper Bound Simulations | 0.04612 | 0.04235 | 0.05096 |
| Any | HCP Cohort | 0.09817 | 0.08464 | 0.11032 |
| | Simulations | 0.08145 | 0.07795 | 0.08570 |
| | Upper Bound Simulations | 0.07579 | 0.07211 | 0.08010 |
