# Supplementary material for: Statistical methods for Mendelian models with multiple genes and cancers
Source: arXiv:2108.12504 ancillary file (2022-05-07)
Supplement: Supplementary file 2 [file figures.pdf]

## Figure Legends

- Figure 1: Associations between the 11 genes, plus a hypothetical PANC gene, (rows) and 11 cancers (columns) collectively incorporated in the PanelPRO models illustrated in this paper. PANC is only listed in order to discuss back-compatibility with PancPRO and is not a gene that can currently be specified in the PanelPRO package. Population-level allele frequencies are given in parentheses (the CHEK2 allele frequency is for the 1100delC only; the allele frequencies for all other genes are for any pathogenic variant). Orange cells correspond to penetrances that are available in the BayesMendel package, and blue cells correspond to penetrances based on a literature review that are also available in ASK2ME.
- Figure 2: AUC, calibration, and MSE for the full PanelPRO-5BC model (black) and the BRCAPRO submodel (blue) evaluated on 1,000,000 families simulated based on PanelPRO-5BC, with (open points) and without (closed points) risk modifiers. “BRCAPRO genes” indicates any of the genes in BRCAPRO (BRCA1, BRCA2), and “Any” indicates any of the five genes in PanelPRO-5BC. 95% bootstrap percentile confidence intervals are also shown.
- Figure 3: AUC, calibration, and MSE for the full PanelPRO-11 model (black) and its BayesMendel submodels BRCAPRO, MMRpro, and Melapro (blue) evaluated on 1,000,000 families simulated based on PanelPRO-11, with (open points) and without (closed points) risk modifiers. “BRCAPRO genes”, “MMRpro genes”, and “Any BM” indicate any of the genes in BRCAPRO (BRCA1, BRCA2), MMRpro (MLH1, MSH2, MSH6), and any model in the BayesMendel package (BRCA1, BRCA2, MLH1, MSH2, MSH6, CDKN2A), respectively. “Any” indicates any of the eleven genes in PanelPRO-11. 95% bootstrap percentile confidence intervals are also shown.
- Figure 4: Area under the curve (AUC) from evaluating PanelPRO-11 on 1,000,000 simulated families plotted against the relative risk of developing each cancer by age 70, for pathogenic variant carriers compared to noncarriers.
- Figure 5: AUC, calibration, and MSE for the full PanelPRO-5BC model (black) and the BRCAPRO submodel (blue) evaluated on the HCP cohort, with (open points) and without (closed points) risk modifiers. “BRCAPRO genes” indicates any of the genes in BRCAPRO (BRCA1, BRCA2), and “Any” indicates any of the five genes in PanelPRO-5BC. 95% bootstrap percentile confidence intervals are also shown.
- Figure 6: AUC, calibration, and MSE for the full PanelPRO-11 model (black) and its BayesMendel submodels BRCAPRO, MMRpro, and Melapro (blue) evaluated on the HCP cohort, with (open points) and without (closed points) risk modifiers. “BRCAPRO genes”, “MMRpro genes”, and “Any BM” indicate any of the genes in BRCAPRO (BRCA1, BRCA2), MMRpro (MLH1, MSH2, MSH6), and any model in the BayesMendel package (BRCA1, BRCA2, MLH1, MSH2, MSH6, CDKN2A), respectively. “Any” indicates any of the eleven genes in PanelPRO-11. 95% bootstrap percentile confidence intervals are also shown.
- Figure 7: Probabilities of carrying a pathogenic variant of any PanelPRO-11 gene plotted against the probabilities for carrying a pathogenic variant of any BRCAPRO gene (BRCA1 or BRCA2, left) and against the probabilities for carrying a pathogenic variant of any MMRpro gene (MLH1, MSH2, or MSH6, right) in the HCP cohort. All counselees shown are true pathogenic variant carriers. BRCA1 or BRCA2 carriers are colored blue; MLH1, MSH2, or MSH6 are colored orange; and carriers of pathogenic variants of any of the six other PanelPRO-11 genes are colored black. Reference lines are drawn at 2.5%.

## Figures

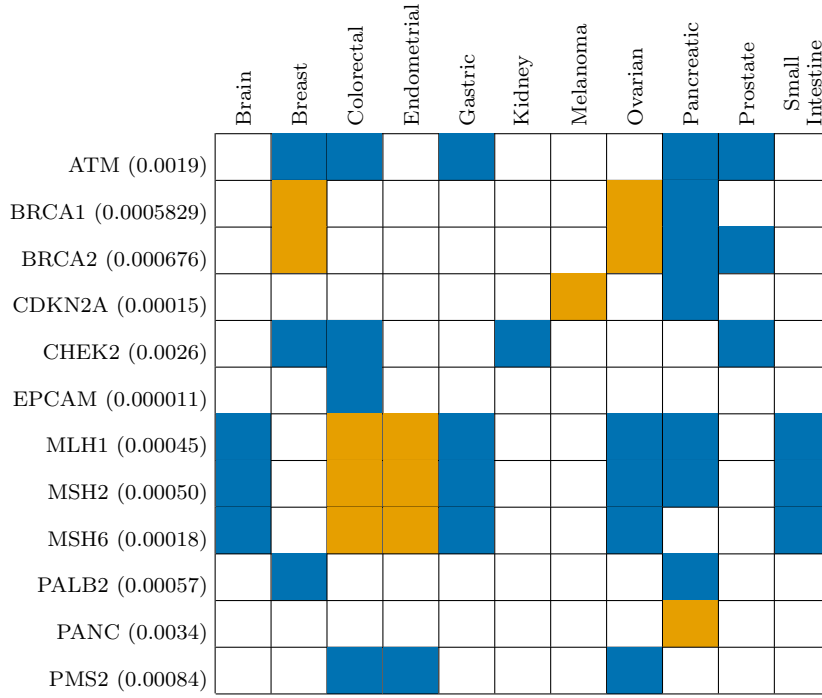

Figure 1: Associations between the 11 genes, plus a hypothetical PANC gene, (rows) and 11 cancers (columns) collectively incorporated in the PanelPRO models illustrated in this paper. PANC is only listed in order to discuss back-compatibility with PancPRO and is not a gene that can currently be specified in the PanelPRO package. Population-level allele frequencies are given in parentheses (the CHEK2 allele frequency is for the 1100delC only; the allele frequencies for all other genes are for any pathogenic variant). Orange cells correspond to penetrances that are available in the BayesMendel package, and blue cells correspond to penetrances based on a literature review that are also available in ASK2ME.

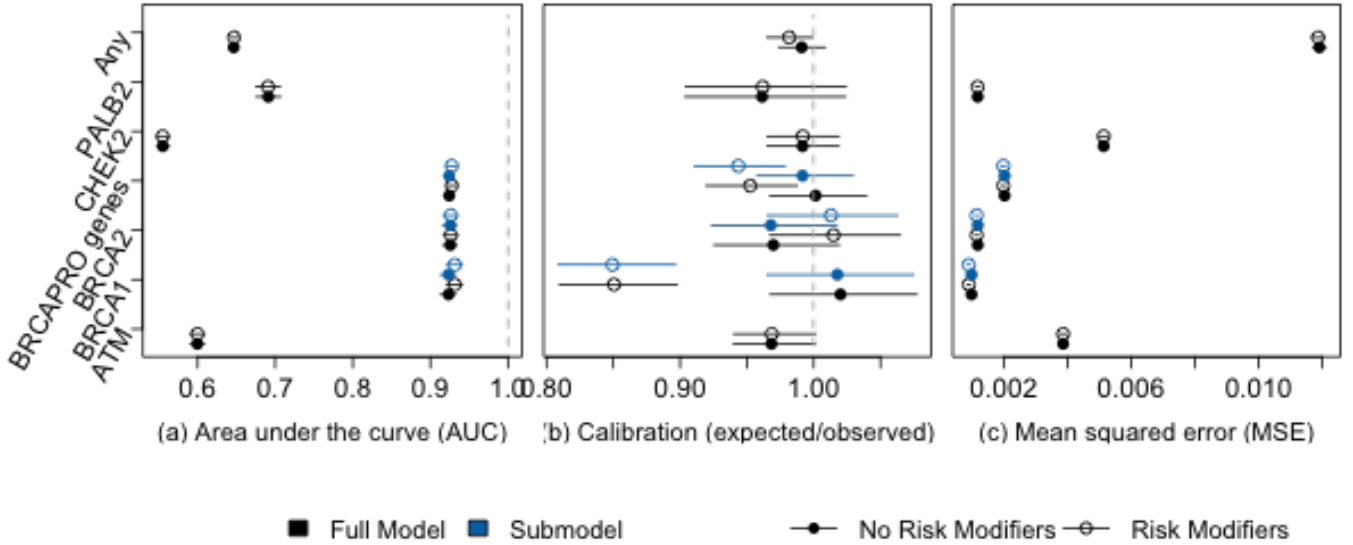

Figure 2: AUC, calibration, and MSE for the full PanelPRO-5BC model (black) and the BRCAPRO submodel (blue) evaluated on 1,000,000 families simulated based on PanelPRO-5BC, with (open points) and without (closed points) risk modifiers. “BRCAPRO genes” indicates any of the genes in BRCAPRO (BRCA1, BRCA2), and “Any” indicates any of the five genes in PanelPRO-5BC. 95% bootstrap percentile confidence intervals are also shown.

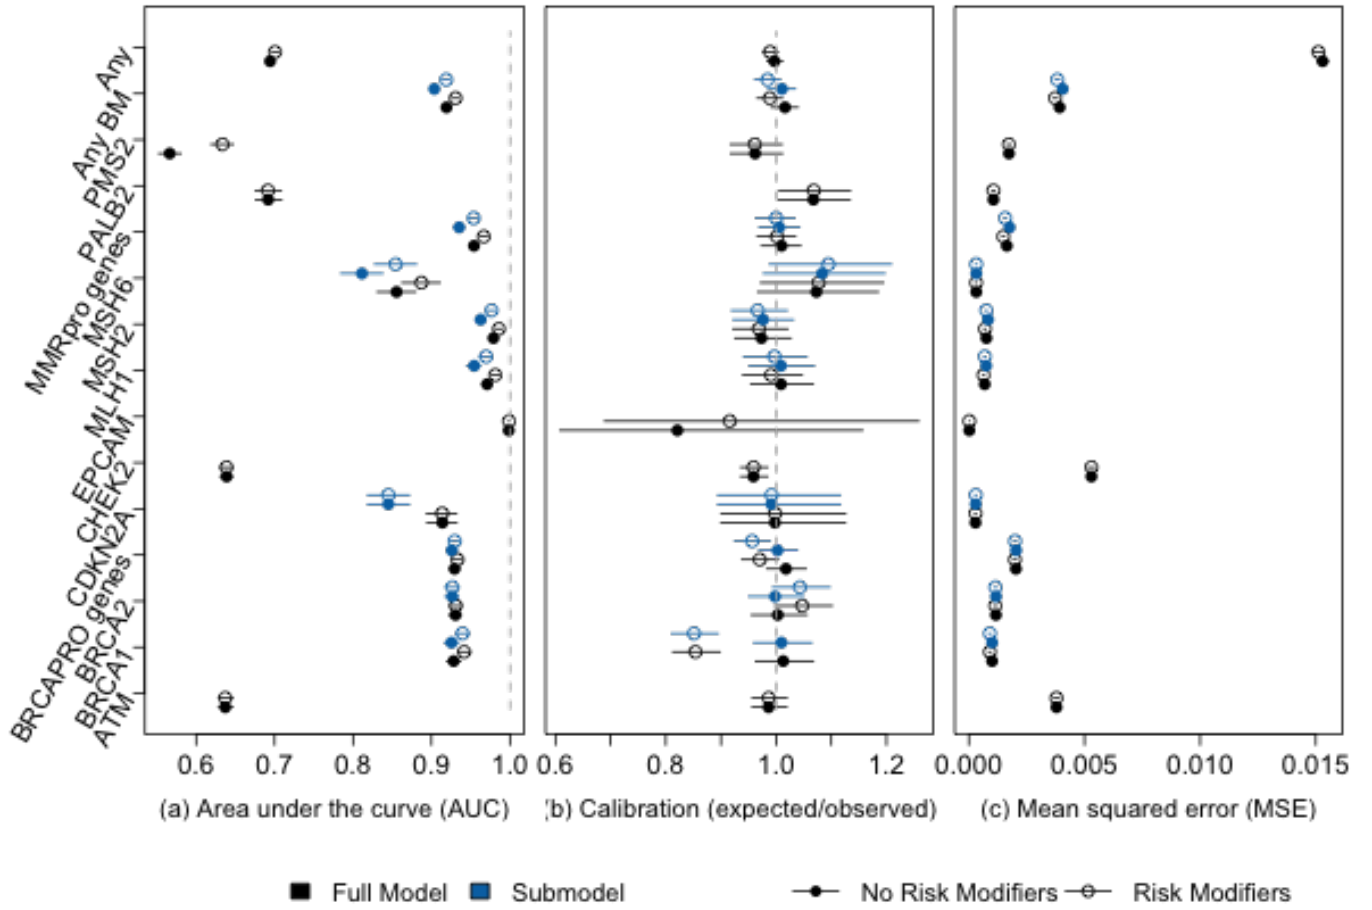

Figure 3: AUC, calibration, and MSE for the full PanelPRO-11 model (black) and its BayesMendel submodels BRCA1, BRCAPRO, and MelapRO (blue) evaluated on 1,000,000 families simulated based on PanelPRO-11, with (open points) and without (closed points) risk modifiers. “BRCAPRO genes”, “MMRpro genes”, and “Any BM” indicate any of the genes in BRCAPRO (BRCA1, BRCA2), MMRpro (MLH1, MSH2, MSH6), and any model in the BayesMendel package (BRCA1, BRCA2, MLH1, MSH2, MSH6, CDKN2A), respectively. “Any” indicates any of the eleven genes in PanelPRO-11. 95% bootstrap percentile confidence intervals are also shown.

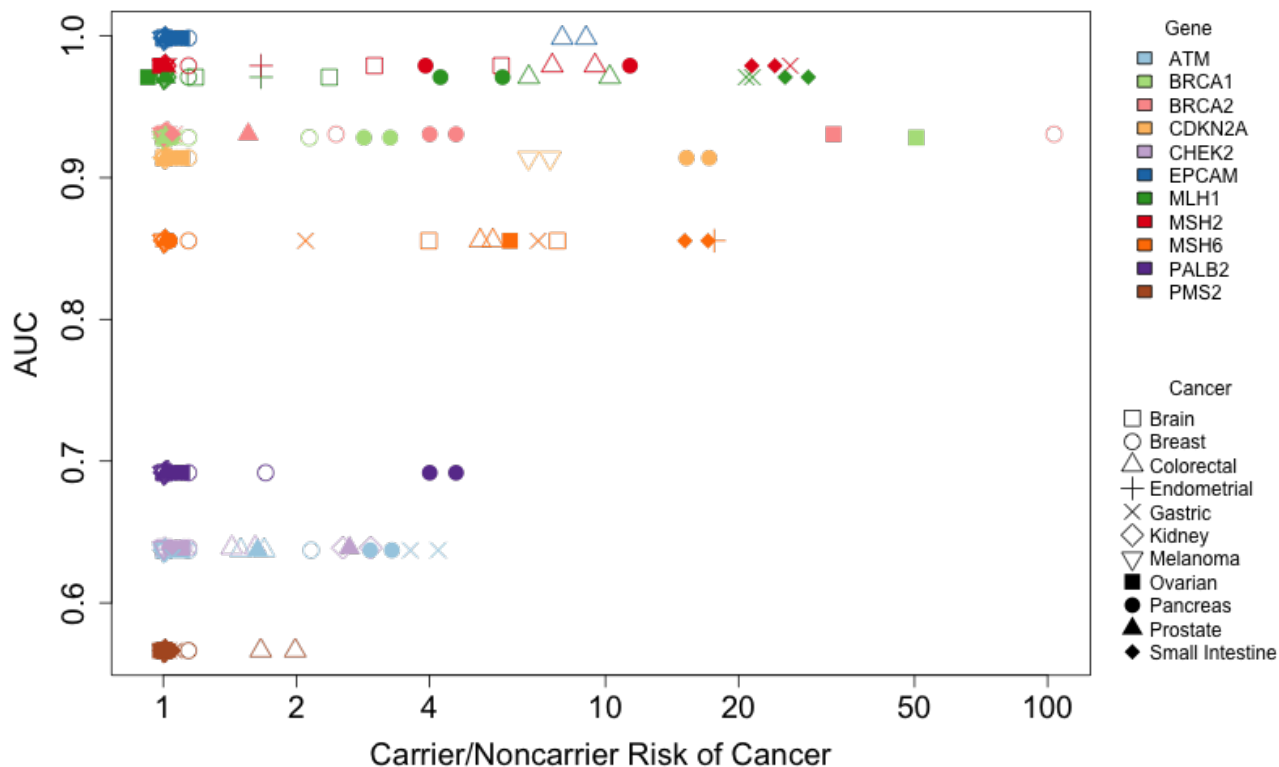

Figure 4: Area under the curve (AUC) from evaluating PanelPRO-11 on 1,000,000 simulated families plotted against the relative risk of developing each cancer by age 70, for pathogenic variant carriers compared to noncarriers.

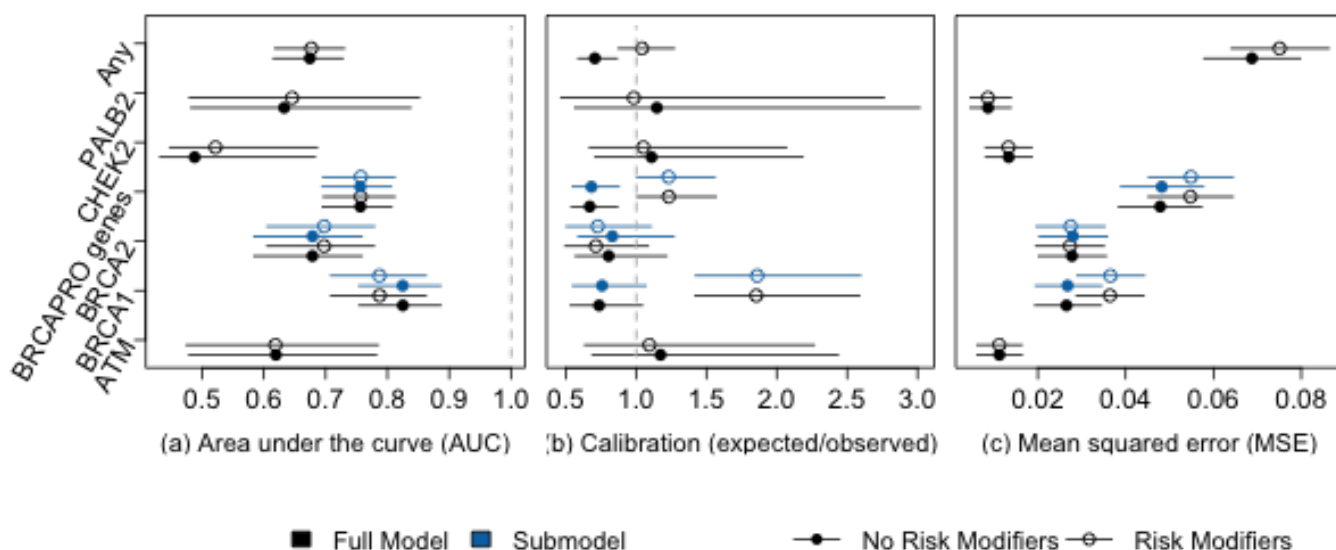

Figure 5: AUC, calibration, and MSE for the full PanelPRO-5BC model (black) and the BRCAPRO submodel (blue) evaluated on the HCP cohort, with (open points) and without (closed points) risk modifiers. “BRCAPRO genes” indicates any of the genes in BRCAPRO (BRCA1, BRCA2), and “Any” indicates any of the five genes in PanelPRO-5BC. 95% bootstrap percentile confidence intervals are also shown.

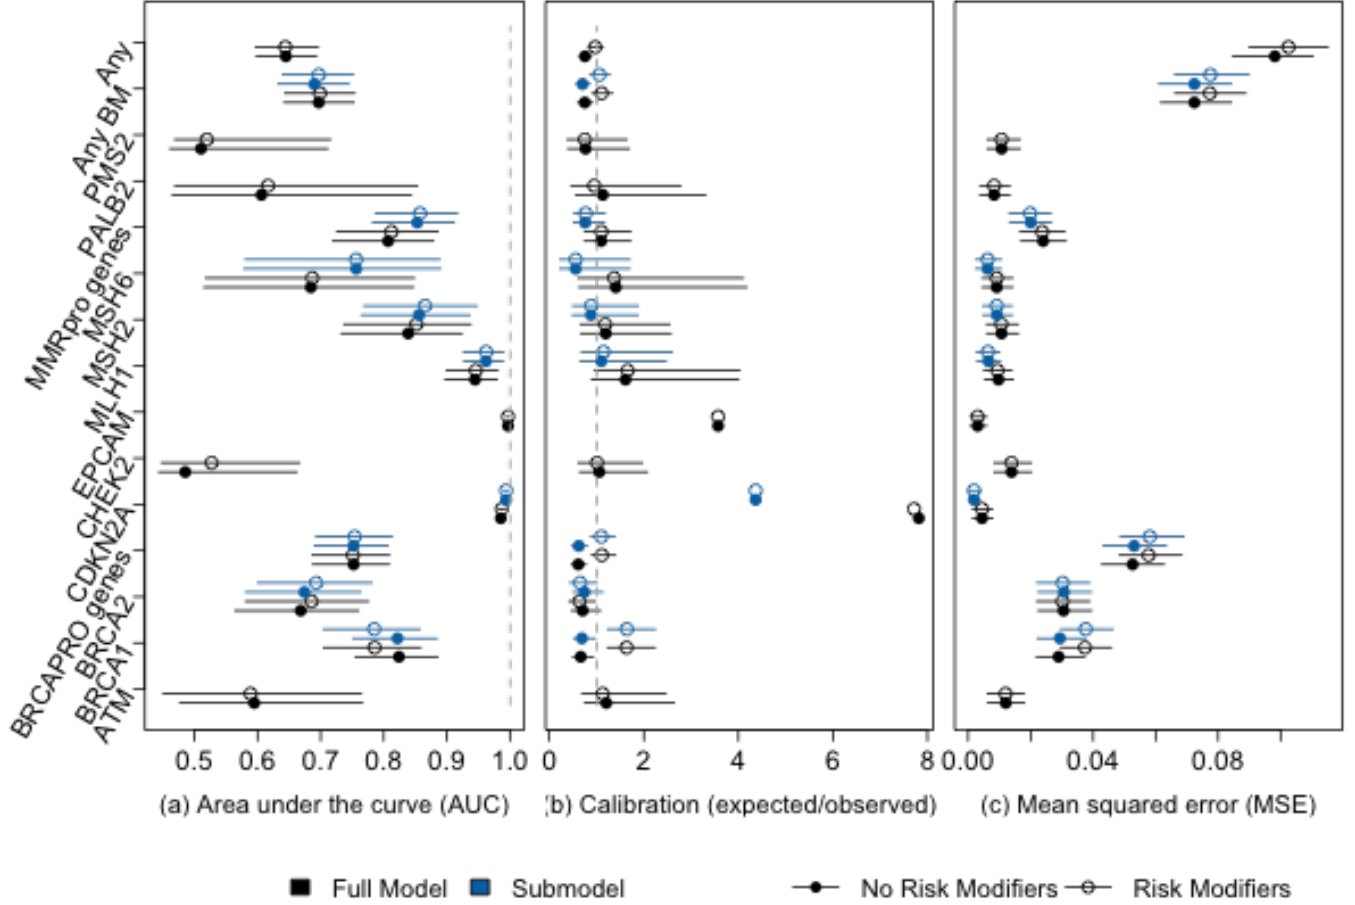

Figure 6: AUC, calibration, and MSE for the full PanelPRO-11 model (black) and its BayesMendel submodels BRCA1, BRCA2, BRCAPRO, MMRpro, and Melapro (blue) evaluated on the HCP cohort, with (open points) and without (closed points) risk modifiers. “BRCAPRO genes”, “MMRpro genes”, and “Any BM” indicate any of the genes in BRCAPRO (BRCA1, BRCA2), MMRpro (MLH1, MSH2, MSH6), and any model in the BayesMendel package (BRCA1, BRCA2, MLH1, MSH2, MSH6, CDKN2A), respectively. “Any” indicates any of the eleven genes in PanelPRO-11. 95% bootstrap percentile confidence intervals are also shown.

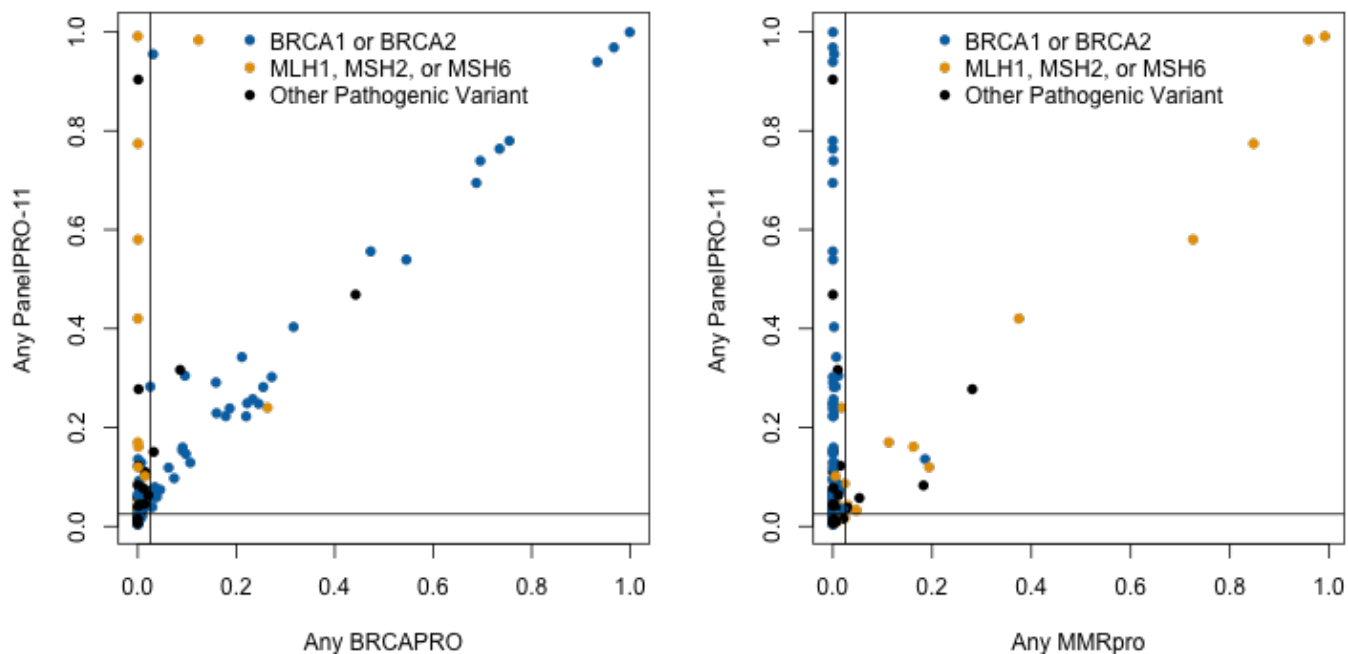

Figure 7: Probabilities of carrying a pathogenic variant of any PanelPRO-11 gene plotted against the probabilities for carrying a pathogenic variant of any BRCA1 or BRCA2 gene (BRCA1 or BRCA2, left) and against the probabilities for carrying a pathogenic variant of any MMRpro gene (MLH1, MSH2, or MSH6, right) in the HCP cohort. All counselees shown are true pathogenic variant carriers. BRCA1 or BRCA2 carriers are colored blue; MLH1, MSH2, or MSH6 are colored orange; and carriers of pathogenic variants of any of the six other PanelPRO-11 genes are colored black. Reference lines are drawn at 2.5%.
